# Supplementary material for: Quantifying echo chamber effects in information spreading over political communication networks
Source: arXiv:1901.03688 ancillary file (2019-07-17)
Supplement: Supplementary file 1 [file SI-SupplementaryInformation.pdf]

# Supplementary Information for "Quantifying echo chamber effects in information spreading over political communication networks"

Wesley Cota,[1] Silvio C. Ferreira,[1,2] Romualdo Pastor-Satorras,[3] and Michele Starnini[4]

[1]*Departamento de Física, Universidade Federal de Viçosa, 36570-900 Viçosa, Minas Gerais, Brazil*
[2]*National Institute of Science and Technology for Complex Systems, Brazil*
[3]*Departament de Física, Universitat Politècnica de Catalunya, Campus Nord B4, 08034 Barcelona, Spain*
[4]*ISI Foundation, via Chisola 5, 10126 Torino, Italy*

## I. ETHICS STATEMENT

The data collection was done using the Python library Twython (available at `https://github.com/ryanmcgrath/twython`) for the connection with the Twitter API, using standard accounts for filtering of public statuses. Only public stream information is released by this API and, therefore, data from users with private profiles (at the time of the collection) are not included in the dataset. The terms, privacy policies and conditions of Twitter were abided by us. All profiles IDs were anonymized before the analysis.

## II. DATA AVAILABILITY

The datasets generated and/or analyzed in this study are available from the corresponding authors on reasonable request.

## III. DATA COLLECTION

We collect data regarding the political discussion on Twitter about the impeachment process of the former president of Brazil Dilma Rousseff [1]. The impeachment process started in December 2nd of 2015 by the acceptance of the president of the Brazilian parliament Eduardo Cunha, and followed a parliamentary recess until February 1st of 2016. The impeachment was officially approved on August 31st of 2016, with a ruling vote in the Senate. During the period of data collection, street protests both against and supporting Dilma Rousseff were arranged within social media particularly in Twitter. A schematic timeline of this process is presented in Table S1.

Our data set is composed of tweets collected daily from the public streaming of the Twitter API by specifying a list of keywords [2] related to the impeachment process along the year 2016. The keywords used in the data mining were selected according to trending topics information and generic words, which were, in principle, related to the impeachment process and that were continuously updated by adding new keywords and keeping the previously added ones. See the list of keywords in Table S2. Keywords were converted to lower case, and their punctuation and accents removed. Tweets have been later filtered according the hashtags they contain, by following the procedure described in Section IV.

We collect tweets from March 5th to December 31st of 2016, by recording the timestamp, user IDs of the sender and mentioned users, and all hashtags contained in each tweet. During this period, we collected a grand total of 48 212 722 tweets, which 12 322 322 of them contained at least one hashtag. The number of tweets with hashtags collected daily is shown in Fig. S1. One can see that such number considerably varies from day to day, with peaks of high activity around some events reported in Table S1. The maximum number of tweets collected containing hashtags in a day was more than 500 thousands, on April 17th, when the parliament voted and approved the impeachment.

Since hashtags are usually employed to express opinions regarding a given topic, in opposition to generic keywords, in our analysis we will focus on the hashtags qualifying the tweets collected.

## IV. HASHTAG CLASSIFICATION

Hashtags can be used to define the political position of the users [3]. To this aim, we define four possible categories for the sentiment $s_t$ of an hashtag used in a tweet $t$: i) not related to the impeachment process ($s_t = \times$), ii) pro-impeachment ($s_t = -1$), iii) anti-impeachment ($s_t = +1$), or iv) neutral ($s_t = 0$). The last one includes tweets whose sentiments are not clearly polarized and hashtags that can express both pro- or anti-impeachment sentiments.

The hashtags were classified by performing a manual annotation of the sentiments they carry [4–7]. Considering the list of the 495 most tweeted hashtags during the collecting process, four volunteers independently performed their categorization. All volunteers were Brazilian, graduated in Physics, and interested in the subject. Two of the authors (WC and SCF) participated

in the analysis. To proceed with the sentiment classification, an interactive webpage (`http://labs.wesleycota.com/twitter`) was used to classify the hashtags according to the four categories. The webpage allowed to browse the Twitter search platform for checking tweets containing the selected hashtag within the time window of interest. The volunteers were instructed to read these tweets before answering the question: "*How do you think that these hashtags were used in tweets related to the process of the impeachment of the president Dilma Rousseff along the year of 2016?*".

The final classification of each hashtag was determined by the majority of the opinions of the volunteers. A number of 321 (64.8%) hashtags had a full agreement, while in 443 (89.5%) of them at least 3 out of 4 persons agreed. Divergent opinions were given for 52 (10.5%) hashtags. The 443 hashtags for which an agreement was achieved are reported in Tables S3 to S5, colored according to their classification: blue for hashtags used in tweets that convey pro-impeachment sentiments, red for anti-impeachment sentiments, grey for neutral sentiments, yellow for not related hashtags. Dark (light) colors have been used to indicate full (partial) agreement. A statistical summary of the classification is presented in Table S6. In Table S7 we report the 52 hashtags for which agreement was not reached. We then extracted the 404 hashtags for which an agreement was achieved as anti-impeachment (200), pro-impeachment (184), or neutral (20) sentiments, and reconstructed the political communication (PC) network described in the main text by filtering out all tweets containing hashtags classified as not related (39) or for which an agreement was not achieved (52). The PC network reconstructed this way is hereafter referred as the `20-neutral` network.

In order to check if the main results are robust with respect to the hashtags classification, we constructed also a different PC network where the 52 hashtags for which an agreement was not achieved were classified as neutral. The corresponding modified `72-neutral` network is defined by 456 hashtags, 72 considered as neutral, with only the remaining 39 classified as not related being filtered out.

## V. RECONSTRUCTION OF THE POLITICAL COMMUNICATION NETWORKS

A total of 48 212 722 tweets were collected using the keyword list. 12 322 322 (25.6%) of them contain at least one hashtag, from which:

- 2 911 655 (23.629%) did not have mentions (text in form @*user*),
- 7 486 459 (60.76%) with at least one hashtag of the `20-neutral` classification,
- 9 908 405 (80.41%) with at least one hashtag of the `72-neutral` classification,
- 74 111 (0.6%) with at least two hashtags of opposite sentiments in the same tweet.

The validity of the hashtag classification method is strengthened by the fact that only 0.6% of the collected tweets have hashtags with opposite sentiments. Only tweets with mentions and at least one hashtag were selected in a first round.

For the case of `20-neutral`, the total number of mentions was 5 050 291, in which 2 327 787 (46.092%) of them were in retweets (RTs). For `72-neutral`, we have 7 596 888 mentions being 3 837 204 (50.510%) in RTs. Discarding RTs, we obtained $N = 285\,670$ users and 2 722 504 explicit mentions for the `20-neutral`, and $N = 437\,728$ users and 3 759 684 explicit mentions for the `72-neutral` network. Hereafter as well as in the main paper, we consider only networks obtained with explicit mentions, i.e., disregarding RTs.

From these filtered datasets, a temporal network $\mathcal{G}$ [8] was constructed, defined by a set of $N$ nodes (users), $\mathcal{N} = \{1, 2, \dots, N\}$. An interaction between node $i$ and node $j$ ($i, j \in \mathcal{N}$) occurs in a time $t$ when the user $i$ mentions user $j$ in a tweet with a sentiment $s_t$. An interaction is represented by a directed temporal link from node $i$ to node $j$ at time $t$, with flavor $s_t$, $e_t = (i, j, t, s_t)$. The set of interactions $\mathcal{E} = \{e_1, e_2, \dots, e_E\}$ forms the sequence of interactions defining the temporal network $\mathcal{G}$. Multiple mentions (to different users) in the same tweet imply multiple simultaneous interactions. It is worth noting that these contacts do not have duration and are not symmetric.

From the temporal network representation $\mathcal{G}$, we extracted a time-aggregated, directed network [9], defining the presence of a static directed link between nodes $i$ and $j$ whenever an interaction between $i$ and $j$ at some point of our observation window has occurred. From this network, we finally extracted the largest strongly connected component (SCC) of the aggregated network [10, 11]. The resulting SCC had $N = 31\,412$ nodes, $L = 833\,123$ links and $W = 1\,552\,389$ interactions in the `20-neutral` network, and $N = 39\,525$ nodes, $L = 1\,063\,699$ links, and $W = 2\,056\,448$ interactions in the case of the `72-neutral` network, see Table S8.

The final temporal networks considered in our analysis were given by the set of users belonging to the SCCs and the explicit interactions among them.

## VI. SENTIMENT ANALYSIS OF TWEETS

Here we present a sentiment analysis of the tweets used to reconstruct the SSC of the PC network. Figs. S2 and S3 show the percentage of daily activity for each sentiment (anti-impeachment, pro-impeachment and neutral) in tweets forming the

20-neutral and 72-neutral networks, respectively. Each sentiment is represented by a different color. Some important dates and events related to the impeachment process, together with the sentiment of the majority of tweets, are indicated in Table S1. For both networks, March 29th had the largest $+1$ activity, when the party PMDB interrupted their support to the Rousseff's government (see Table S1). The activity of pro-impeachment sentiments ($-1$) was larger in the June 4th and July 29th, when Rousseff presented her final defense in the Deputy's chamber.

## VII. NETWORK PROPERTIES

The reconstructed PC networks can be represented as a temporal network, in terms of the set of interactions $\{e_t\}$, or in terms of a static aggregated network, which is directed and weighted in nature. The static network is given by the adjacency matrix $\mathcal{A} = \{A_{ij}\}$ in which $A_{ij} = 1$ if $i$ ever interacted with the user $j$, forming a directed link from $i$ to $j$, or 0 otherwise; and by the weight matrix $\mathcal{W} = \{W_{ij}\}$ in which $W_{ij}$ is the total number of directed interactions between $i$ and $j$. The total number of links is denoted as

$$L = \sum_{ij} A_{ij}, \tag{1}$$

while the total number of interactions is

$$W = \sum_{ij} W_{ij}. \tag{2}$$

For each node $i$, we define the out-degree as

$$k_{\text{out},i} = \sum_{j} A_{ij}, \tag{3}$$

the in-degree as

$$k_{\text{in},i} = \sum_{j} A_{ji}, \tag{4}$$

and the degree as

$$k_i = \sum_{j} \tilde{A}_{ij}, \tag{5}$$

where $\tilde{A}_{ij} = 1$ if $i$ has mentioned $j$ or vice-versa (undirected) at least once in the time window.

The activity of a sender $a_i$ or receiver $a_i^{\text{IN}}$ are defined as

$$a_i = \sum_{j} W_{ij} \text{ and } a_i^{\text{IN}} = \sum_{j} W_{ji}, \tag{6}$$

such a way that the total activity (number of tweets exchanged) is $a_i^{\text{total}} = a_i + a_i^{\text{IN}}$.

The distributions of activity $\rho(a)$ for the two PC networks are shown in Fig. S4. In all cases, the activity distributions exhibit heavy tails, compatible with a power law form $\rho(a) \sim a^{-\alpha}$. This indicates that, while the average activity can be small, a non-negligible fraction of users can send or receive a disproportionately large number of tweets. If we restrict the analysis to users with activity between $a \in [10, 100]$ we have that activity is approximately homogeneous across different political position levels as can seen in Fig. S5. The political position $P$ is defined in the main paper.

The main average properties of the PC networks are summarized in Table S8, in which data for both SCC and whole networks are presented.

The PC networks have a marked community structure [12], that can be obtained by applying the Louvain algorithm [13], based in the partition of the networks in groups of nodes, such that the modularity $Q$, defined by

$$Q = \frac{1}{2m} \sum_{ij} \left( \tilde{A}_{ij} - \frac{k_i k_j}{2m} \right) \delta(g_i, g_j) \tag{7}$$

is maximized. In Eq. (7), $m = \sum_{ij} \tilde{A}_{ij}$ is the number of links in the undirected network and $g_i$ is the group to which node $i$ belongs. This resulted in $Q = 0.435$ and 0.431 for the 20-neutral and 72-neutral networks, respectively. The community structures of both networks are described in Table S9.

## VIII. ANALYSIS OF THE `72-NEUTRAL` NETWORK

Figures S6 to S9 reproduce for the `72-neutral` network the results corresponding to to `20-neutral` network in Figures 1 to 4 in the main paper. We see essentially the same behavior for both `20-neutral` and `72-neutral`.

## IX. AVERAGE POLITICAL POSITION OF THE PREDECESSORS

Figure S10 presents a contour map for the average political position of the predecessors $P_{\rm in}^{\rm NN}$ as a function of the political position $P$. It shows the same behavior as the corresponding plot for successors shown in Figure 2(a) in the main paper.

## X. NUMBER OF RETWEETS AS FUNCTION OF THE POLITICAL POSITION

Figure S11 shows an analysis of the number of RTs a user achieves, as a function of his/her political position and activity. We observe that the number of RTs is quite clearly correlated with the activity of a user, which is a natural result: a more active user sends more tweets, and thus have chances to get a larger total number of RTs. The average number of RTs per activity appears to be quite uncorrelated with the political position.

## XI. ANALYSIS OF THE SPREADING MODELS FOR DIFFERENT PARAMETERS

Figure S12 presents supplementary heat maps for the average spreadability $\langle S \rangle$ obtained with the SIS model as function of the political position $P$ and the activity $a$ for different values of the infection probability.

In Figs. S13 and S14, analysis of the dependence with the infection rate and healing times of the average spreadability $\langle S \rangle$, diversity $\sigma$, and political position $\mu$ of the set of influence $\mathcal{I}$ are shown for SIS and SIR epidemic processes, respectively. We can see that despite expected quantitative differences due to the nature of models, both dynamical processes exhibit similar behaviors which are also preserved as the parameters are varied.

Figure S15 shows the effects of different activity intervals used in the analysis with the same parameters of Figure 4 in the main paper.

## XII. RELATION BETWEEN POLITICAL POSITION AND TOPOLOGY

Figure S16 presents the average $k$-core index [14] and the average degree (Eq. 5) as function of the political position $P$. In both analyses, we see the same pattern observed for activity as function of $P$ shown in Fig. S5(a). This behavior deviates from that of spreadability as function of $P$, showing that such topological quantities are not able to fully explain the spreadability dependence on $P$.

## XIII. RESULTS FOR THE WATTS THRESHOLD MODEL

In order to check the robustness of our results on different spreading models, we have considered additionally a modification of the classic Watts threshold model of complex contagion [15]. In this model, each individual is either in state $S$ or $I$, whose interpretation is akin to the one in the SIR/SIS models. We have considered the absolute-threshold version of the Watts model on temporal networks described in Ref. [16], in which each individual is endowed with a threshold value $\Phi$. For each interaction at a time $t$, an individual in state $S$ counts the total number of contacts from infected vertices to him/her within a time window $[t-\theta, t]$. If this value is larger than $\Phi$, individual $i$ flips to state $I$; otherwise it remains in the $S$ state. Transitions from $I$ to $S$ are forbidden. Starting from a single individual in state $I$, a cascade of transitions to state $I$ is produced. In Fig. S17 we show the results analogous to those for SIS and SIR models using the absolute-threshold Watts model to compute spreadability and diversity as function of the political position $P$. As we can observe, all three models yield the same qualitative behavior.

## XIV. SUPPLEMENTARY TABLES

Tables S1 to S9 report important facts concerning the impeachment process of president Rousseff as well as details of the communication network reconstruction process.

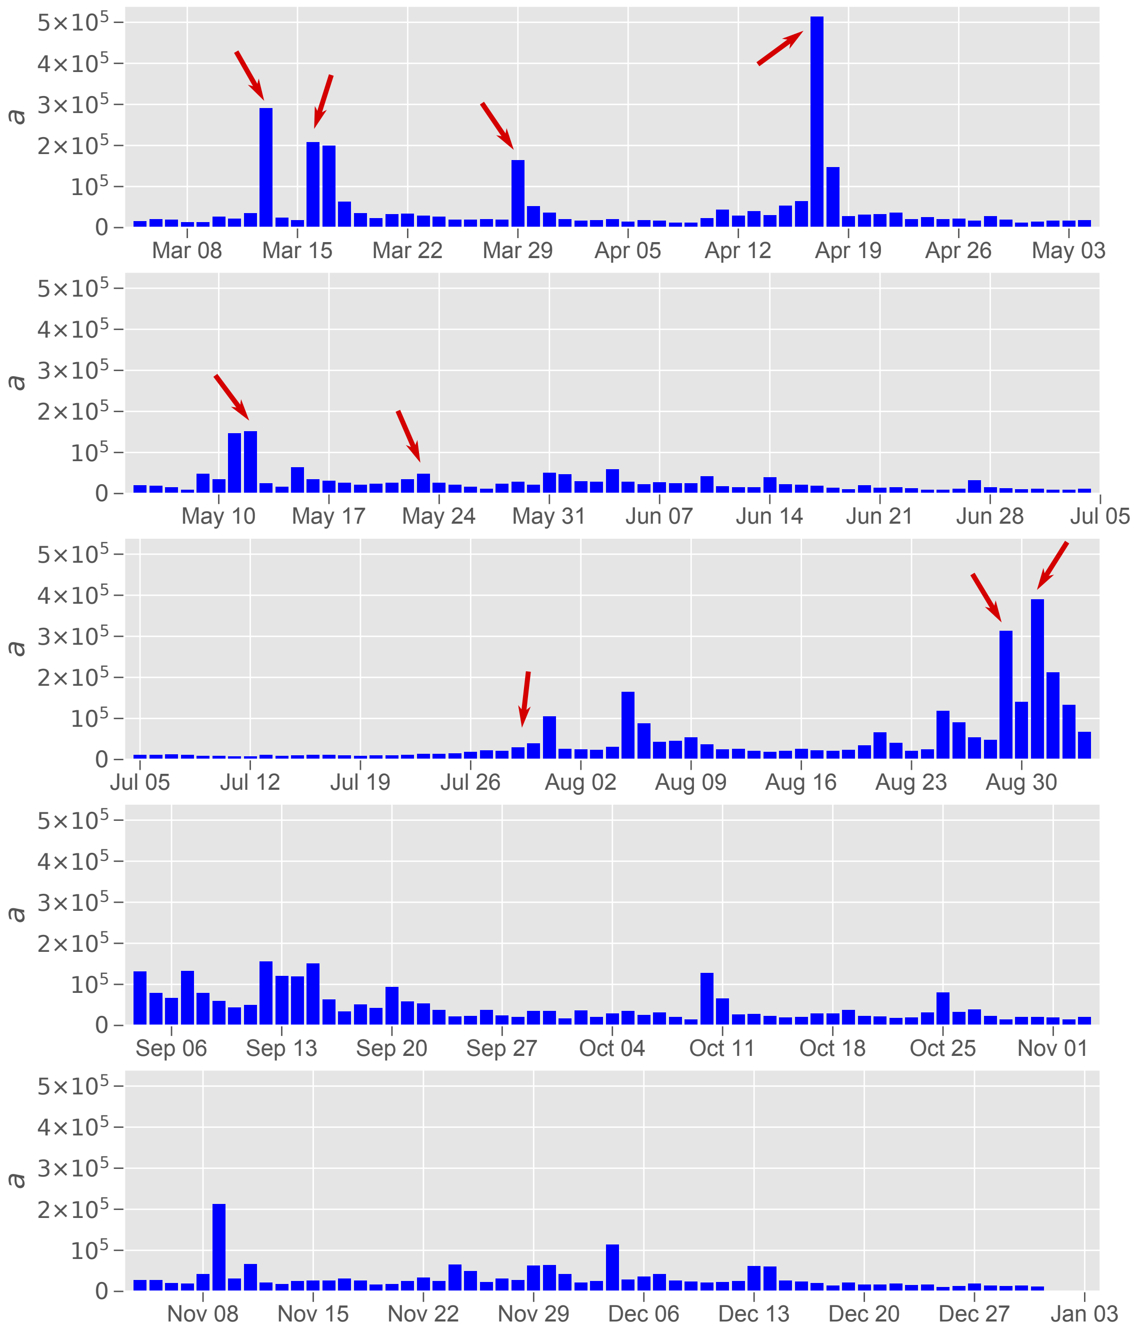


FIG. S1. Activity of tweets with hashtags collected as function of the day. High activity can be observed around some events, reported in Table S1, which are indicated by arrows. The high activity in November 9th coincide with Trump's victory in USA election which is, in principle, not related to the process we are investigating. This peak of activity disappears when we consider only the largest strongly connected component of the communication network. Arrows indicate the relevant political events singled out in Table S1.

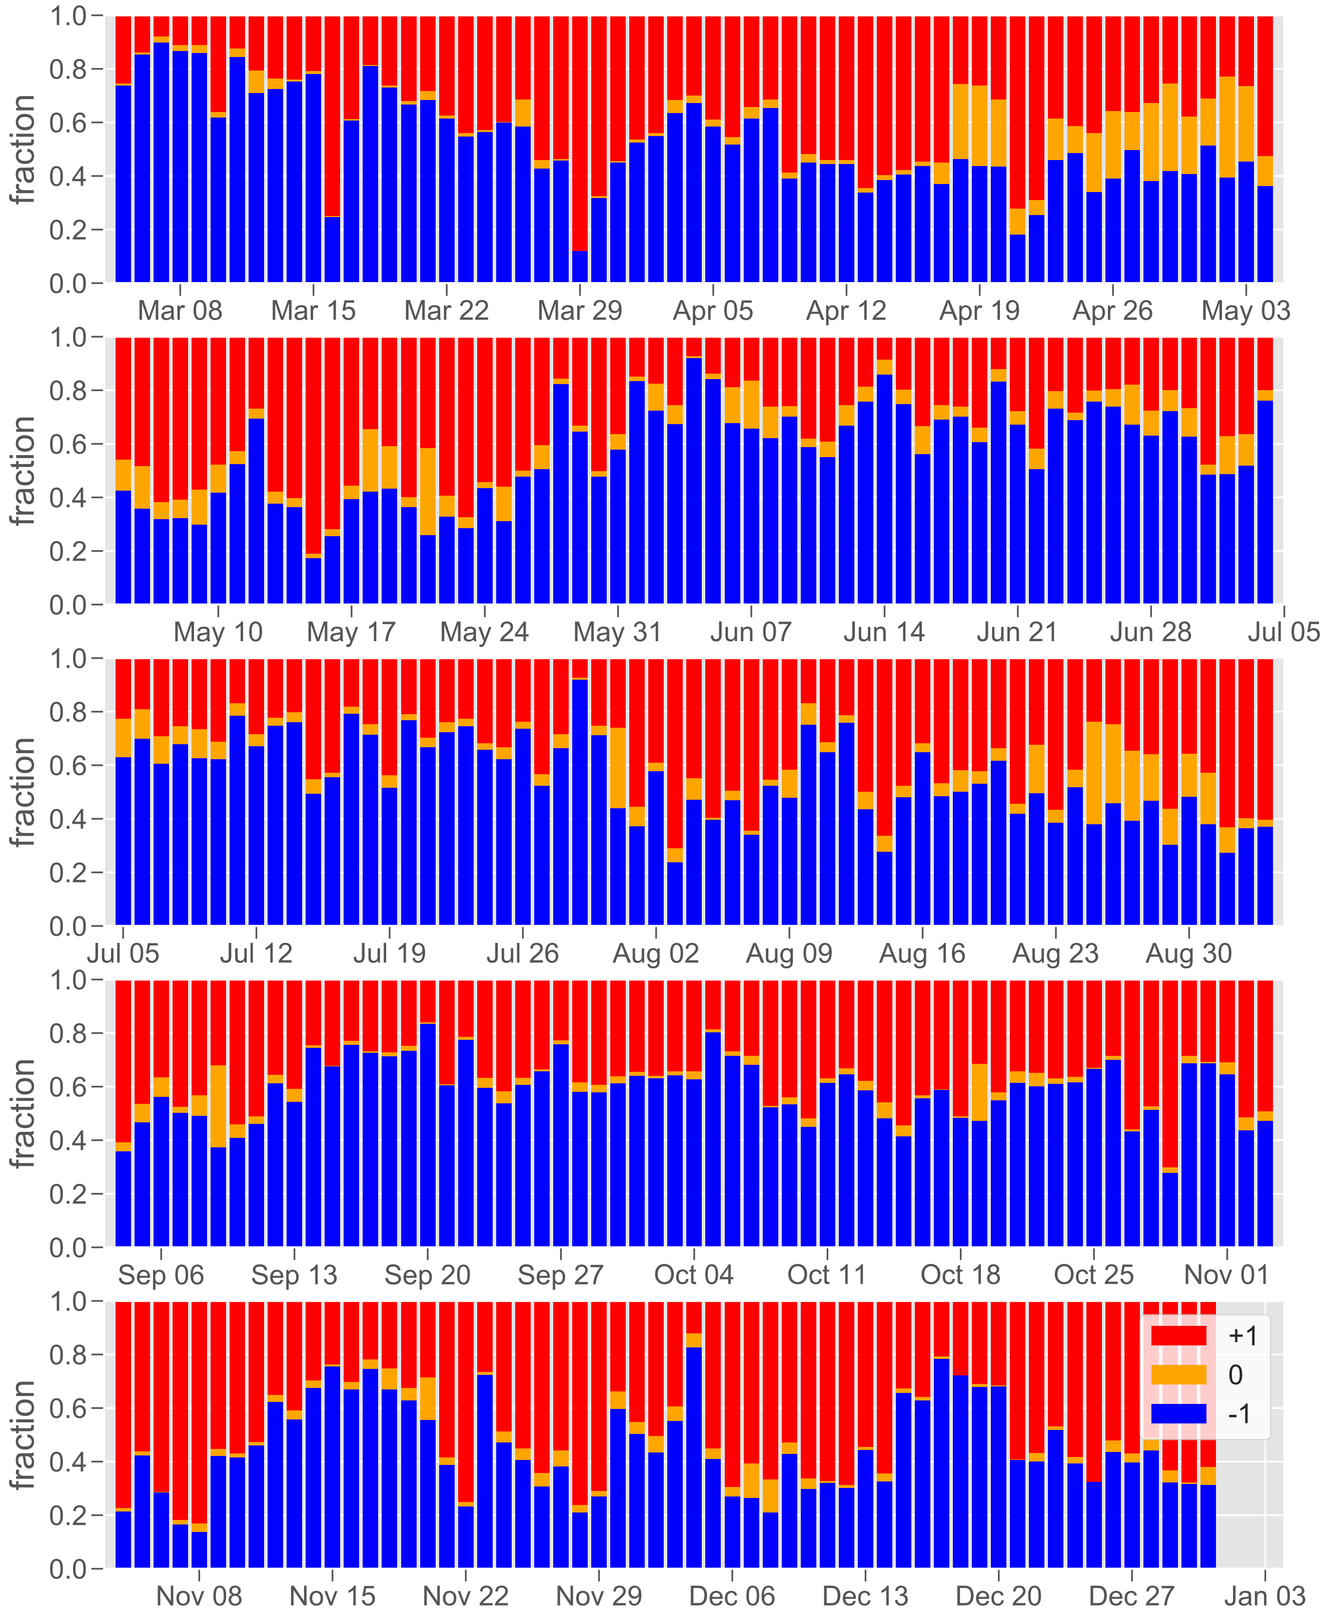


FIG. S2. Activity frequency of tweets for the SCC of the `20-neutral` network. The legend indicates the colors corresponding to the activity for $-1$, $0$ and $+1$ interactions.

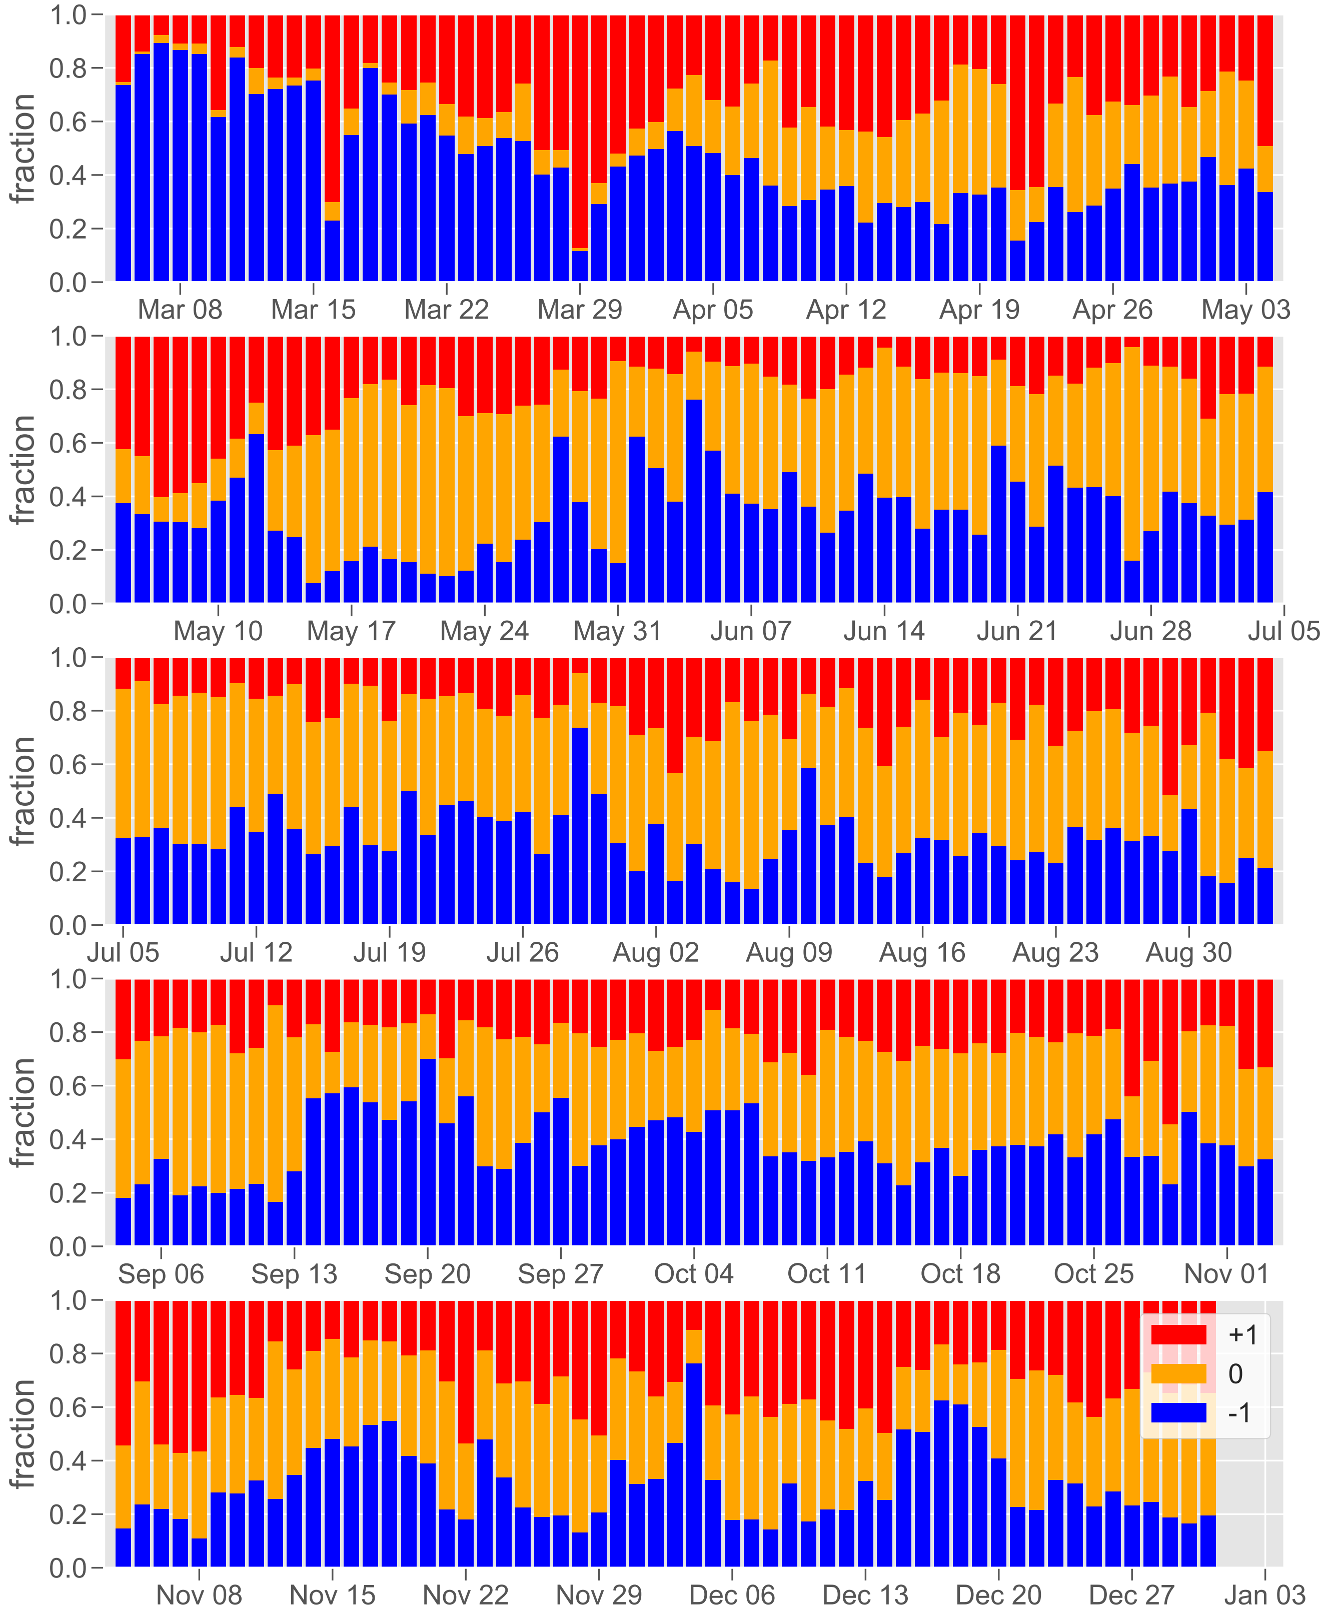


FIG. S3. Activity frequency of tweets for the SCC of the `72-neutral` network. The legend indicates the colors corresponding to the activity for $-1$, 0 and $+1$ interactions.

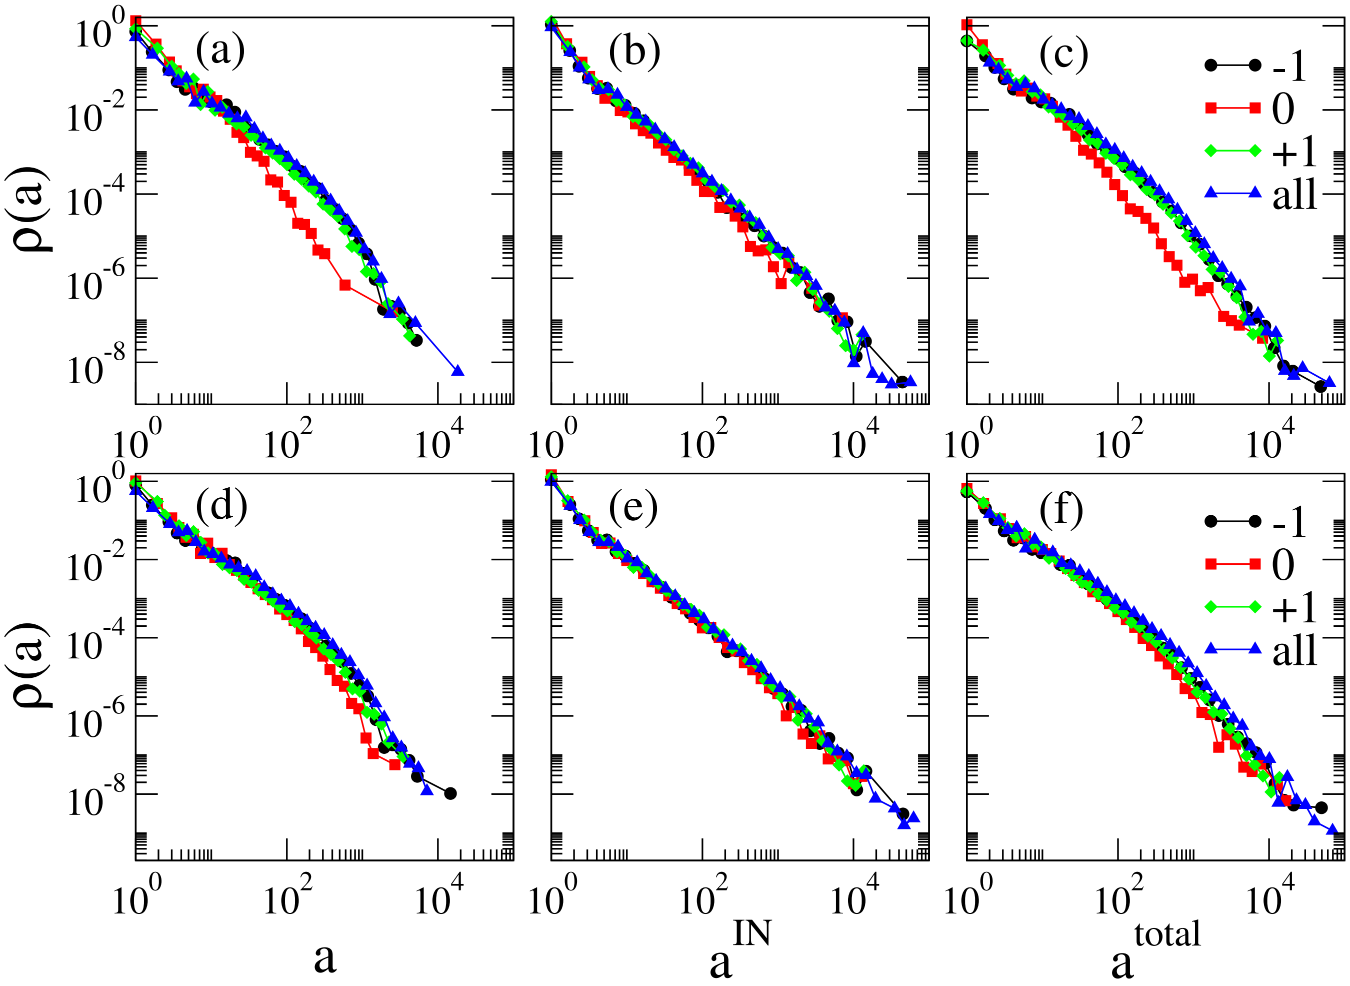


FIG. S4. Distributions of (a,d) activity of sender $\rho(a)$, (b,e) receiver $\rho(a^{\mathrm{IN}})$ and (c,f) total activity $\rho(a^{\mathrm{total}})$ of interactions with sentiments $-1$, 0, $+1$ and all tweets. The top row corresponds to `20-neutral` and the bottom to `72-neutral` networks.

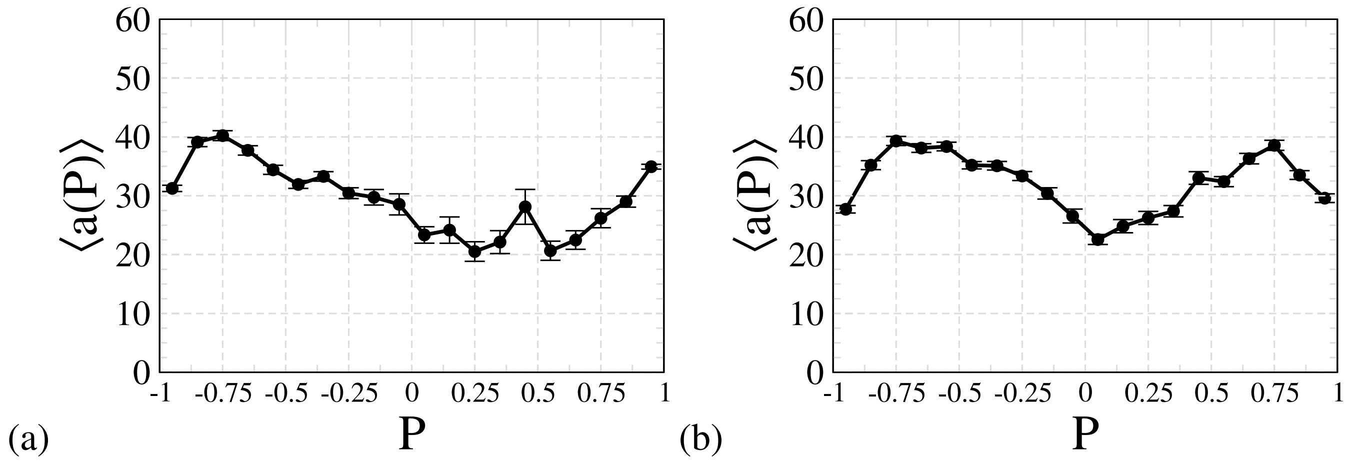


FIG. S5. Average activity versus political position for users with activity $a \in [10, 100]$ for (a) `20-neutral` and (b) `72-neutral` PC networks. Error bars represent the standard error.

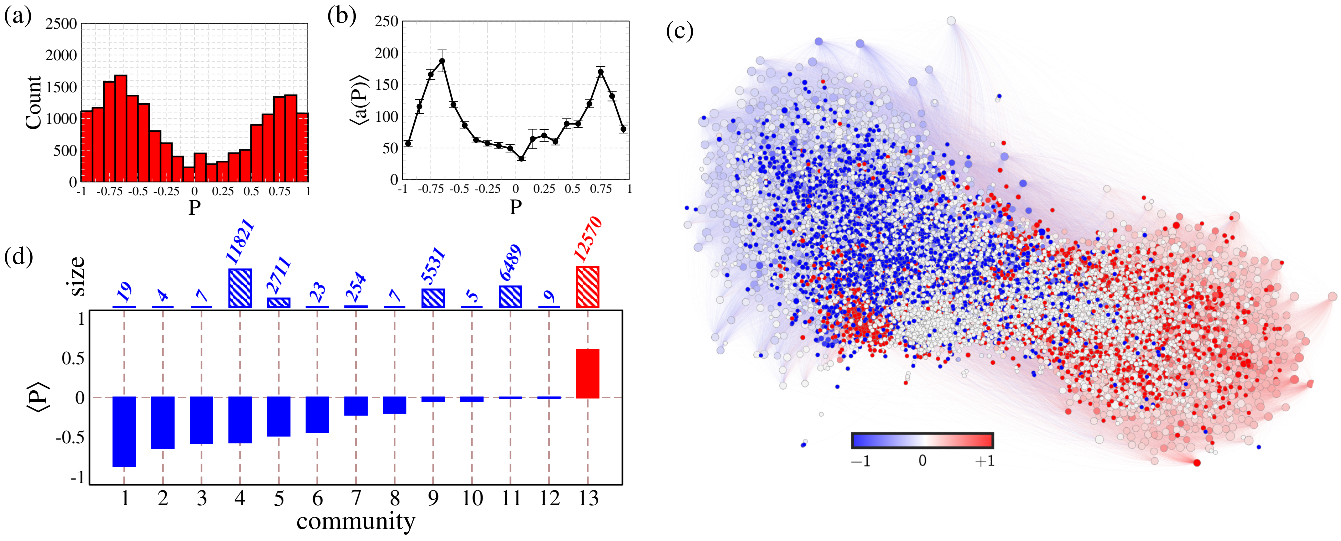


FIG. S6. Figure 1 of the main paper for the `72-neutral` network. (a) Number of users as a function of political position $P$. (b) Average activity as function of $P$. Only users with activity $a \geq 10$ in the SCC are considered for (a) and (b). (c) Visualization of the time-aggregated representation of the PC network, formed by $N = 39\,525$ users in the SCC. The size of nodes increases (non-linearly) with their degree. Colors represent political position, as defined in the main paper, blue for pro-, red for anti-impeachment, and white for neutral average sentiment of users. (d) Community size and average political position of different communities identified by the Louvain algorithm.

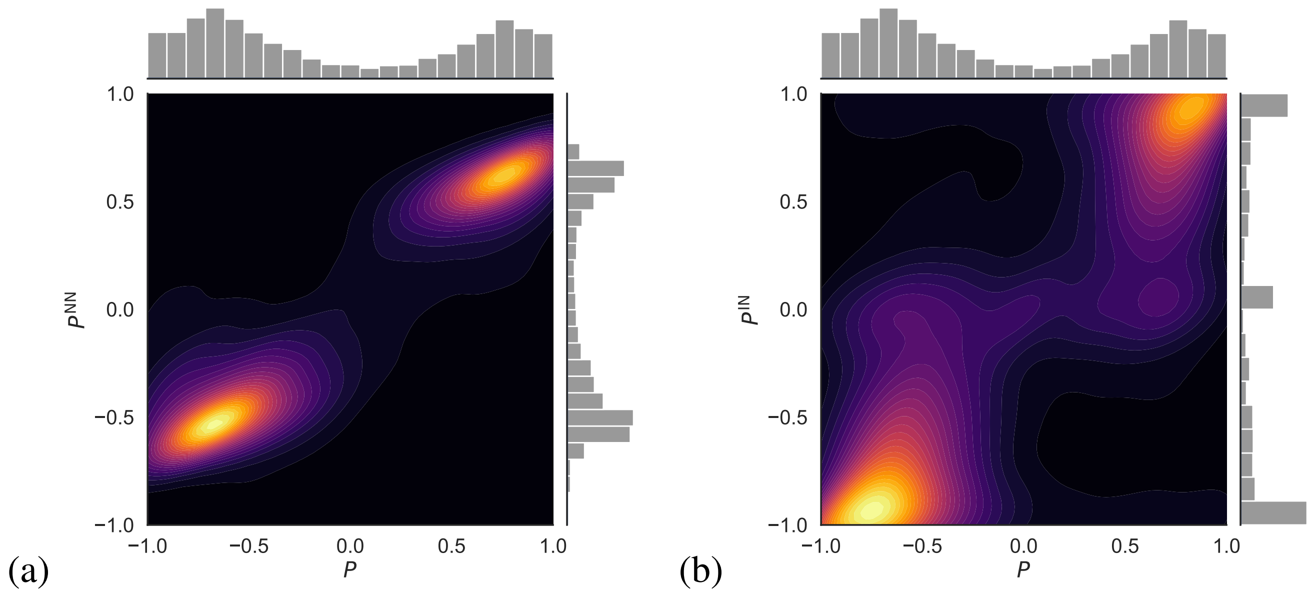


FIG. S7. Figure 2 of the main paper for the `72-neutral` network. Contour maps for the (a) average political position $P$ of the nearest-neighbor $P^{\mathrm{NN}}$ and (b) average sentiment of received tweets, $P^{\mathrm{IN}}$ against $P$. Colors represent the density of users: the lighter the larger the number of users. Probability distribution of $P$, $P^{\mathrm{NN}}$, and $P^{\mathrm{IN}}$ are plotted in the axes. Only users with activity $a \geq 10$ (corresponding to 17923 users) are considered.

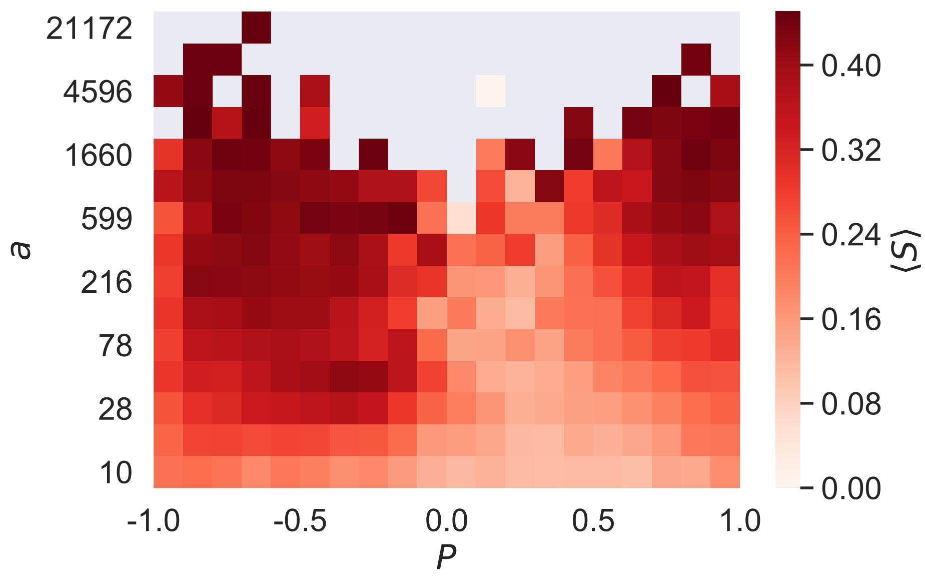


FIG. S8. Figure 3 of the main paper for the `72-neutral` network. Heat map of the average spreadability $\langle S \rangle$ of users, as a function of their political position $P$ and activity $a$. The transmission probability of the SIS dynamics is $\lambda = 0.5$ and $\tau = 7$ days. Averages were performed over 100 runs.

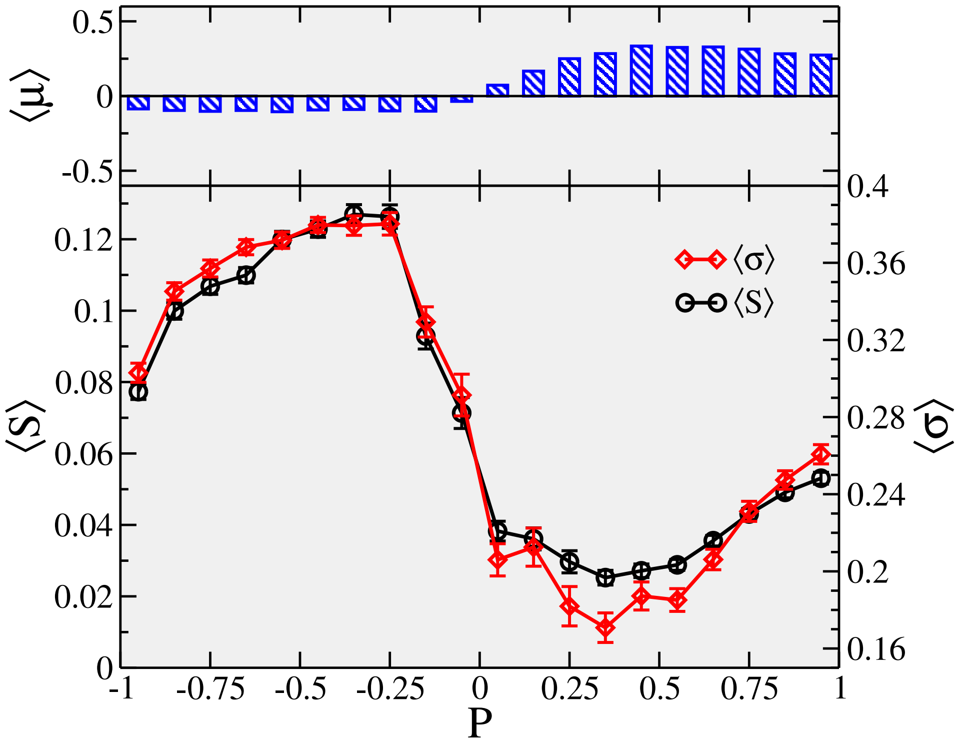


FIG. S9. Figure 4 of the main paper for the `72-neutral` network. Average spreadability $\langle S(P) \rangle$ (black curve, left axes), diversity $\langle \sigma(P) \rangle$ (red curve, right axes) and political position $\langle \mu(P) \rangle$ (bars, top panel) of the set of influence reached by users with political position $P$. Transmission probability $\lambda = 0.2$ and $\tau = 7$ days. Only the 13556 users with activity $a \in [10, 100]$ are considered. Results are averaged over 100 runs, error bars represent the standard error.

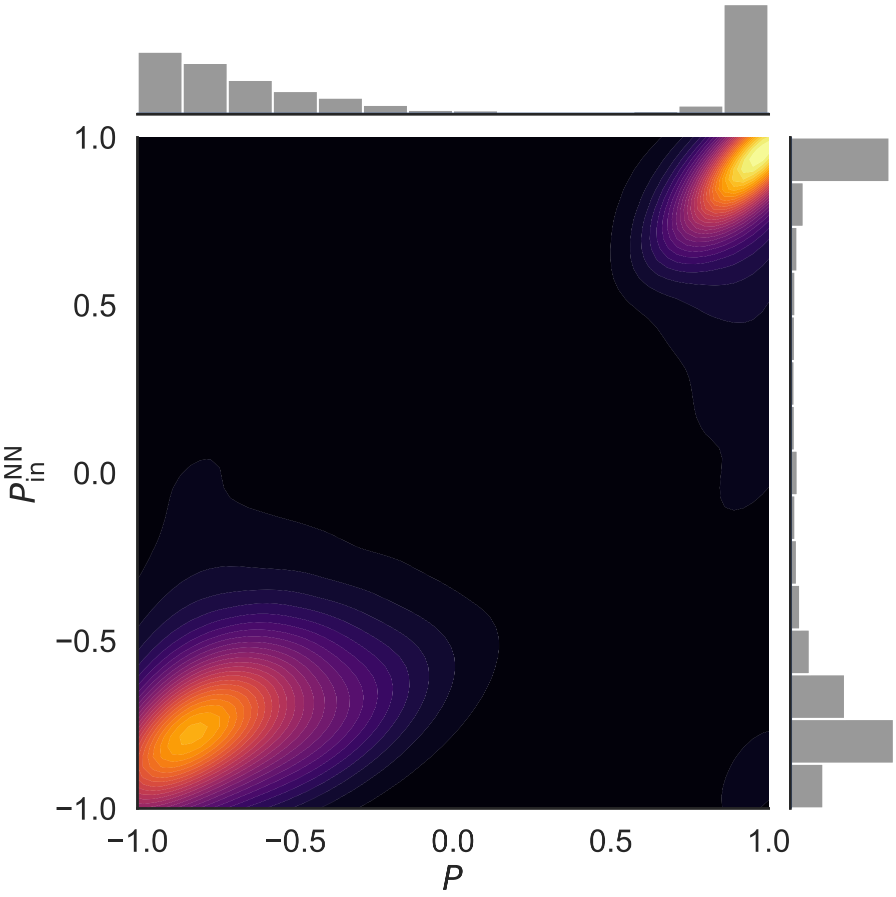


FIG. S10. Contour maps for the average political position of the predecessors $P_{\rm in}^{\rm NN}$, given by $P_{{\rm in},i}^{\rm NN} \equiv \sum_j A_{ji} P_j / k_{{\rm in},i}$, against the political position $P$ of a user for the `20-neutral` network. The political position $P$ is defined in the main text. Colors represent the density of users: the lighter the larger the number of users. Probability distribution of $P$ and $P^{\rm NN}$ are plotted in the axes. Only users with activity $a \geq 10$ (corresponding to 14813 users) are considered.

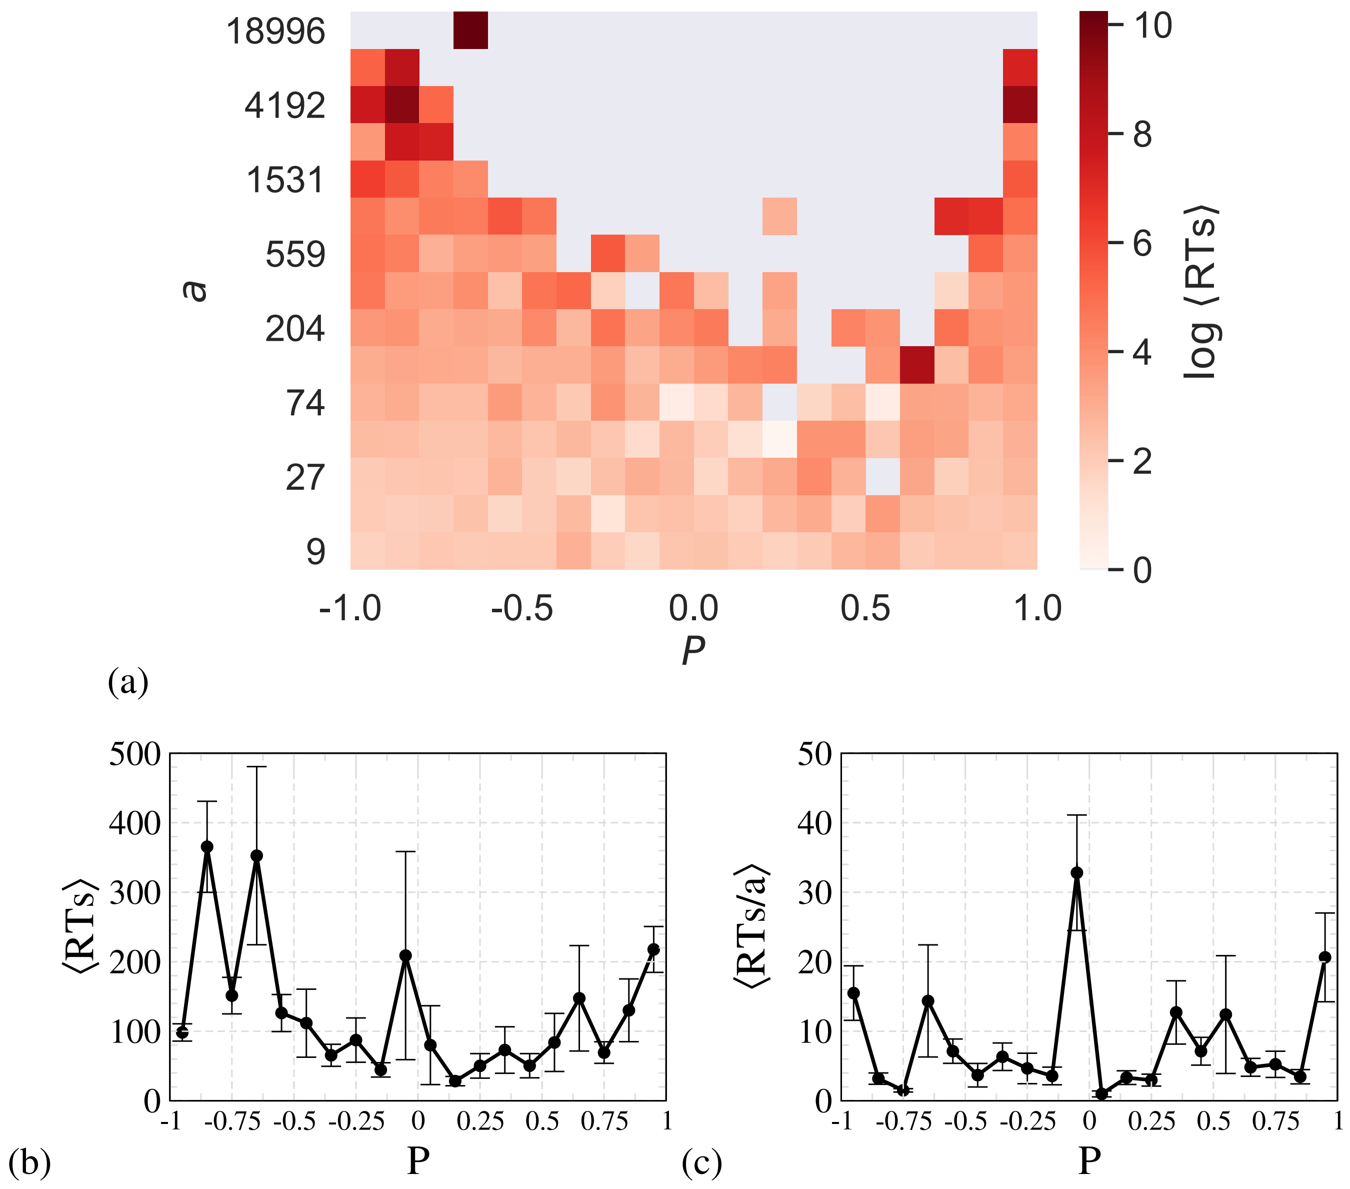


FIG. S11. Number of retweets received by users of the `20-neutral` network in the classified data: (a) heat map of the number of retweets of users as a function of their political position $P$ and activity $a$, (b) average number of retweets and (c) average number of retweets normalized by the user activity as function of the political position. Error bars represent the standard error.

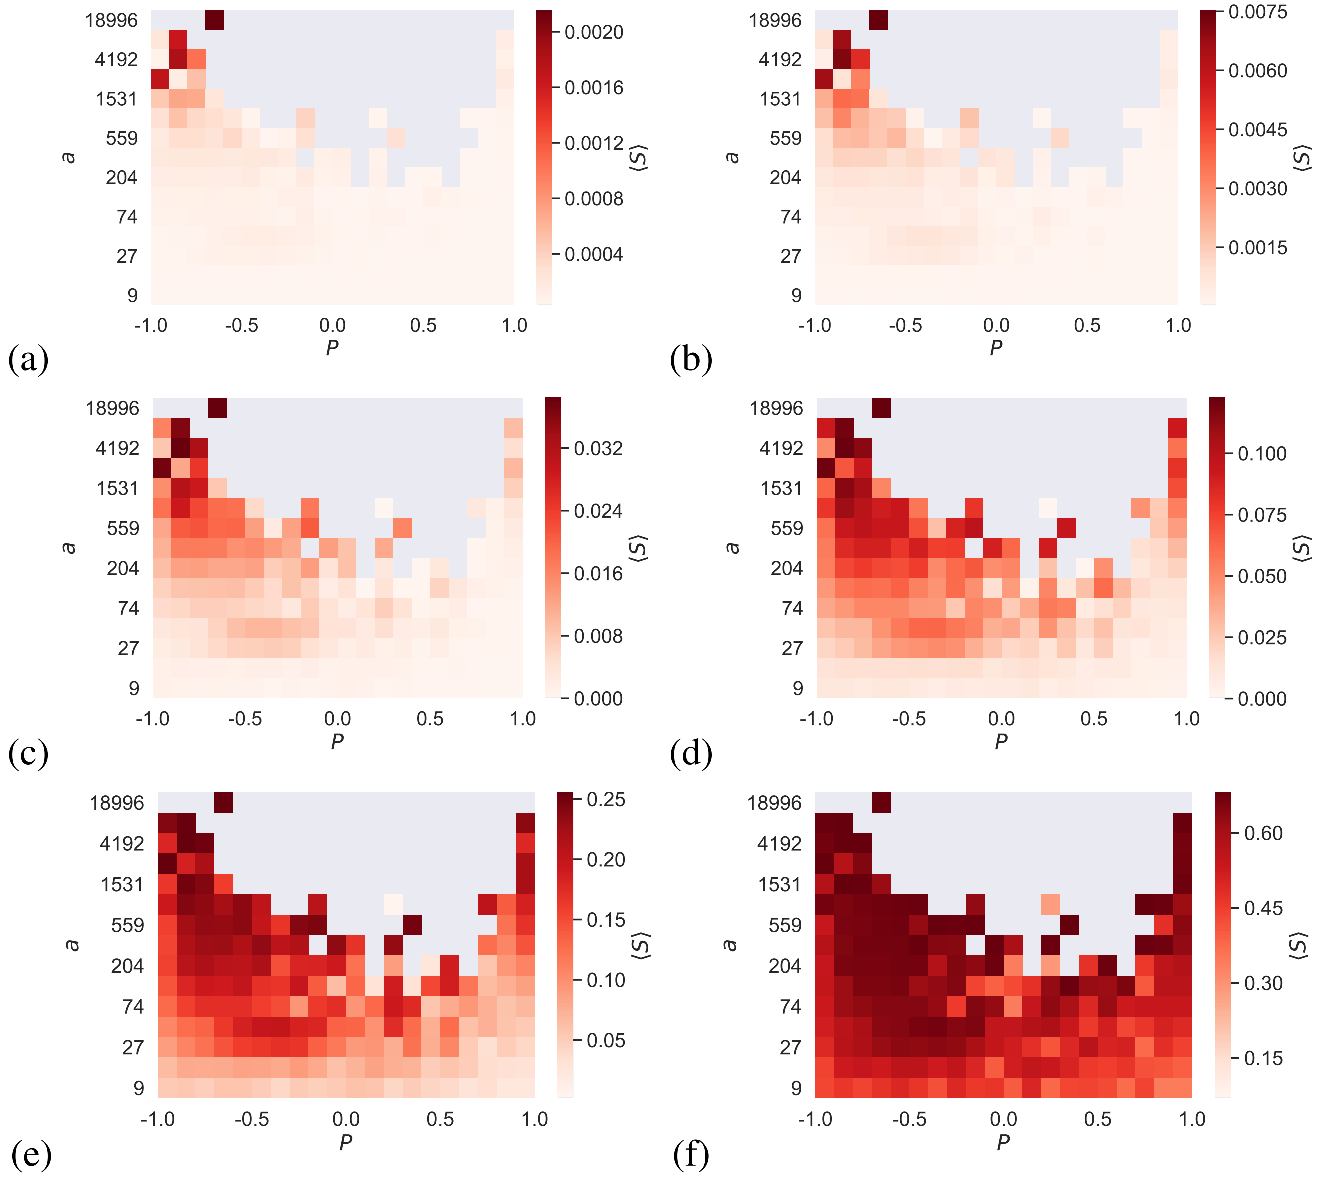


FIG. S12. Heat maps of the average spreadability $\langle S \rangle$ of users generated with the SIS model as a function of their political position $P$ and activity $a$ for temporal network with healing time $\tau = 7$ days for the `20-neutral` network and transmission probability (a) $\lambda = 0.01$, (b) $\lambda = 0.02$, (c) $\lambda = 0.05$, (d) $\lambda = 0.1$, (e) $\lambda = 0.2$, and (f) $\lambda = 1$. The case $\lambda = 0.5$ is presented in the main text. Averages were performed over 100 runs.

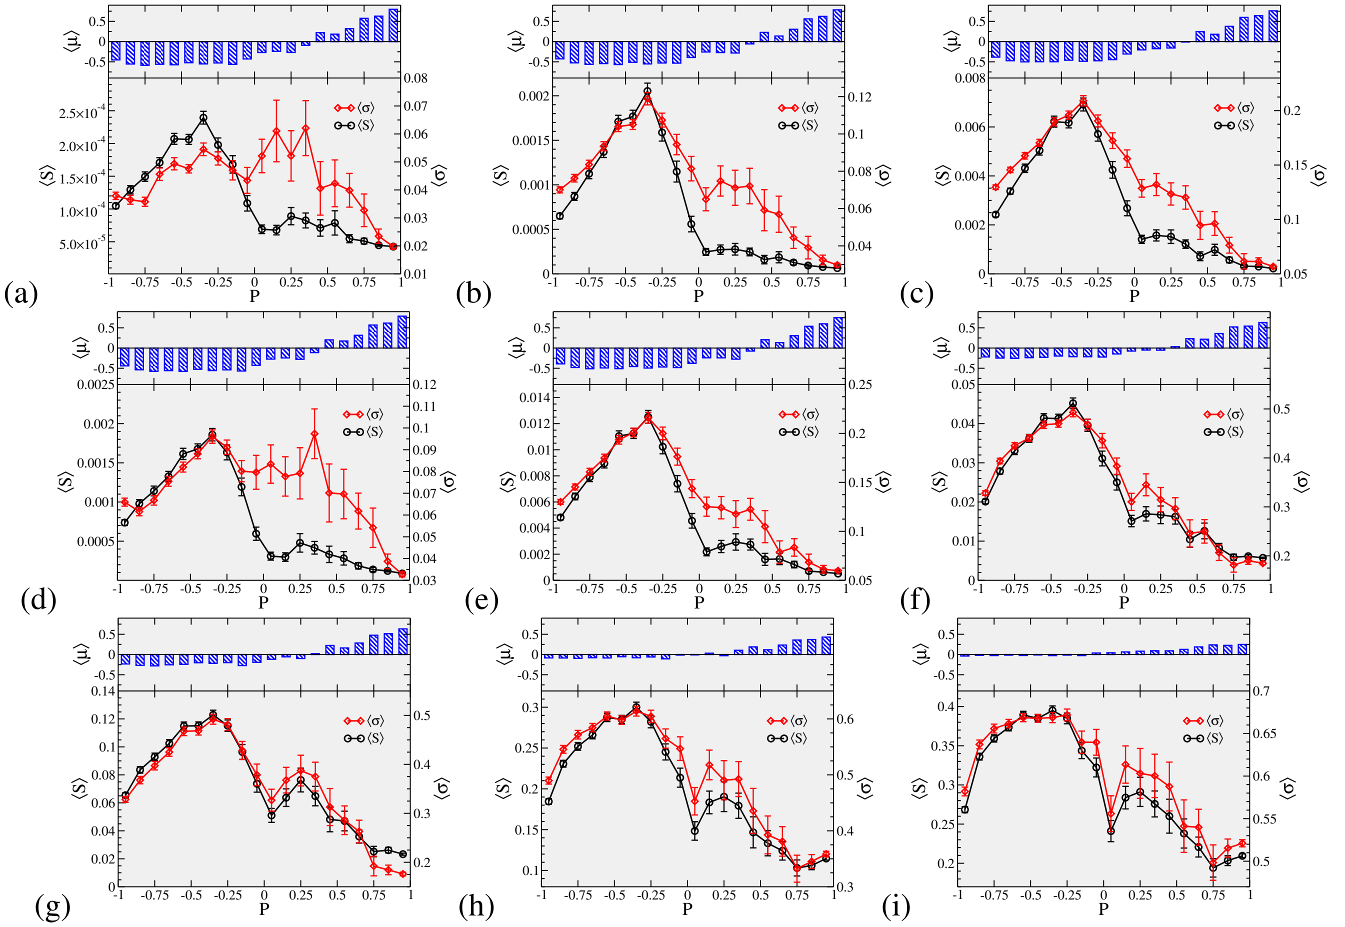

FIG. S13. Average spreadability $\langle S \rangle$ (black, left axes), diversity $\sigma$ (red, right axes), and political position $\mu$ (top panel) of the set of influence $\mathcal{I}$, as a function of the political position $P$, for SIS model with transmission probability (a)–(c) $\lambda = 0.05$, (d)–(f) $\lambda = 0.10$ and (g)-(i) $\lambda = 0.50$ for the temporal `20-neutral` network. The healing times $\tau$ are (a,d,g) 1 day, (b,e,h) 3 days and (c,f,i) 7 days. Only users with activity $a \in [10, 100]$ were considered. Averages were performed over 100 runs.

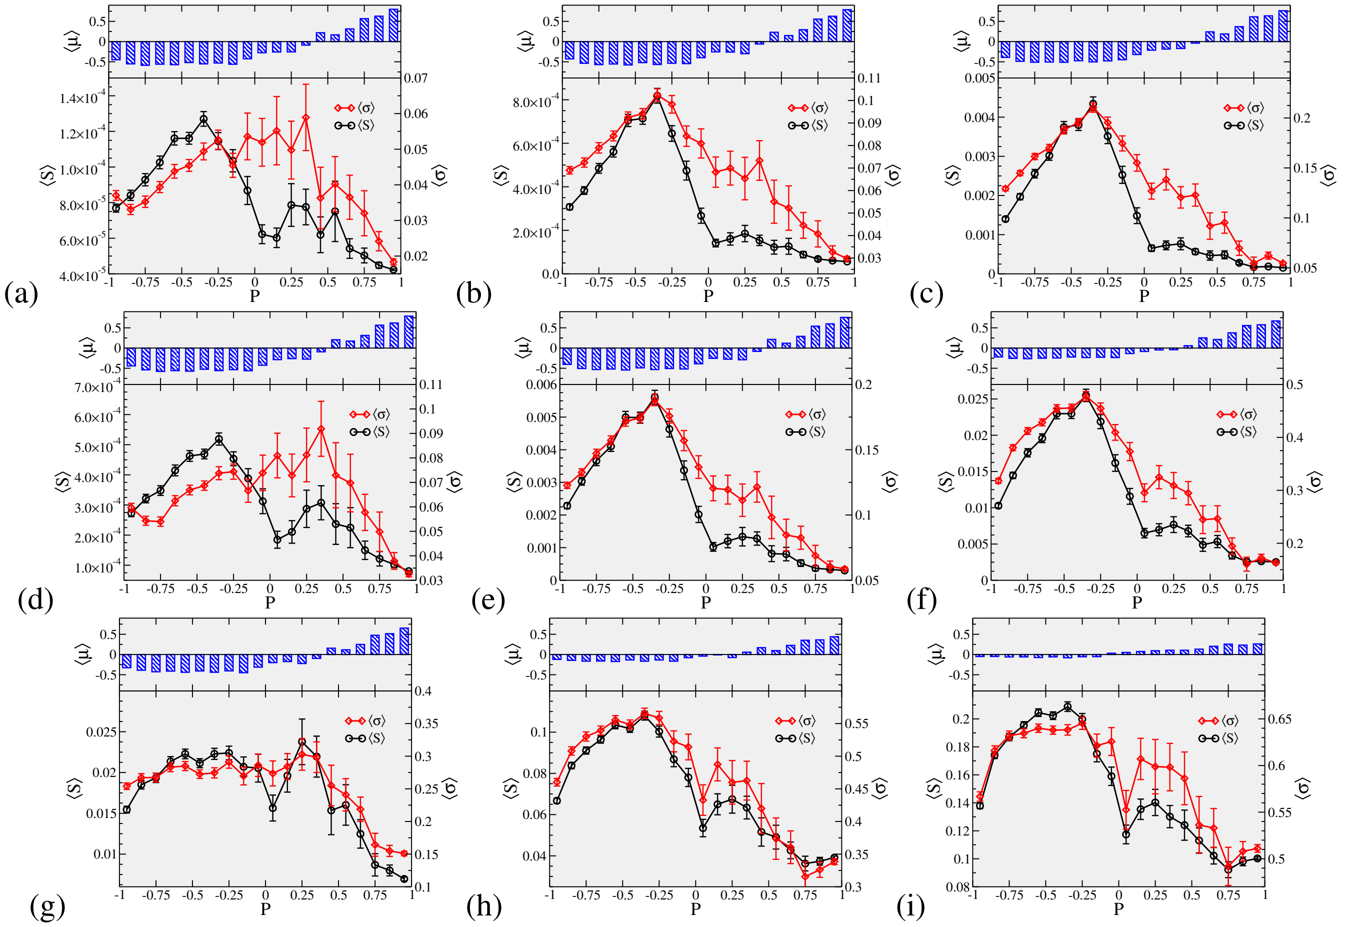


FIG. S14. Average spreadability $\langle S \rangle$ (black, left axes), diversity $\sigma$ (red, right axes), and political position $\mu$ (top panel) of the set of influence $\mathcal{I}$, as a function of the political position $P$, for SIR model with transmission probability (a)–(c) $\lambda = 0.05$, (d)–(f) $\lambda = 0.10$ and (g)-(i) $\lambda = 0.50$ for the temporal `20-neutral` network. The healing times $\tau$ are (a,d,g) 1 day, (b,e,h) 3 days and (c,f,i) 7 days. Only users with activity $a \in [10, 100]$ were considered. Averages were performed over 100 runs.

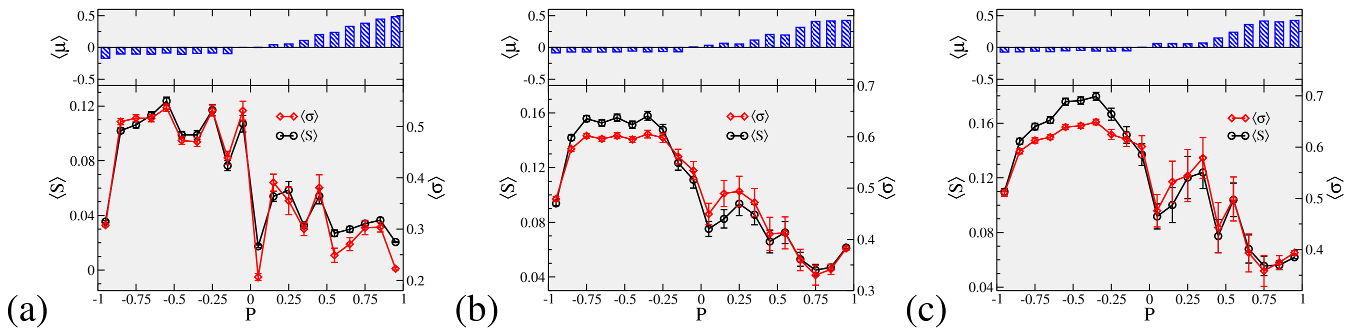


FIG. S15. Average spreadability $\langle S \rangle$ (black, left axes), diversity $\sigma$ (red, right axes), and average political position $\mu$ (top panel) of the set of influence $\mathcal{I}$, as a function of the political position $P$, for SIS model with transmission probability $\lambda = 0.2$ and $\tau = 7$ days for the temporal `20-neutral` network. Only users with activity (a) $a \in [1, 100]$, (b) $a \in [10, 500]$ and (c) $a \in [20, 200]$ are considered, in a total of 27985, 14313 and 10409 users, respectively. Fig. 4 of the main paper shows results for $a \in [10, 100]$. Averages were performed over 100 runs.

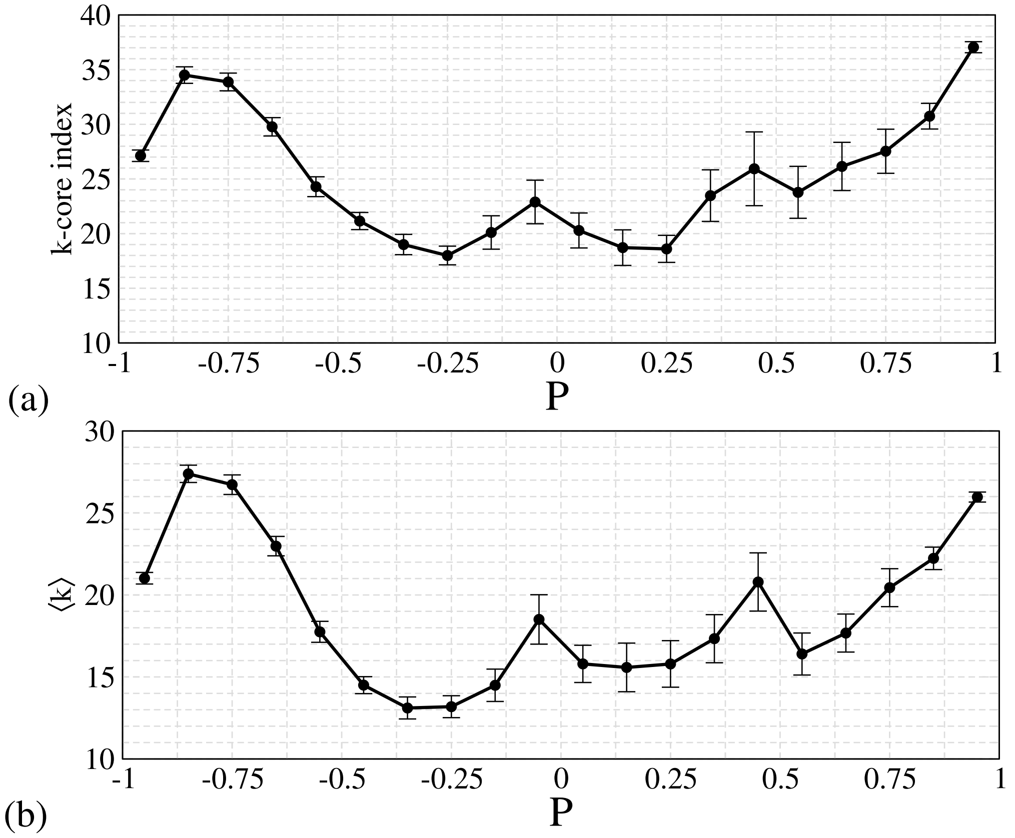


FIG. S16. Topological centrality measures as function of political position $P$ for the `20-neutral` network: (a) average $k$-core index and (b) average degree as functions of the political position. Only users with activity $a \in [10, 100]$ are considered.

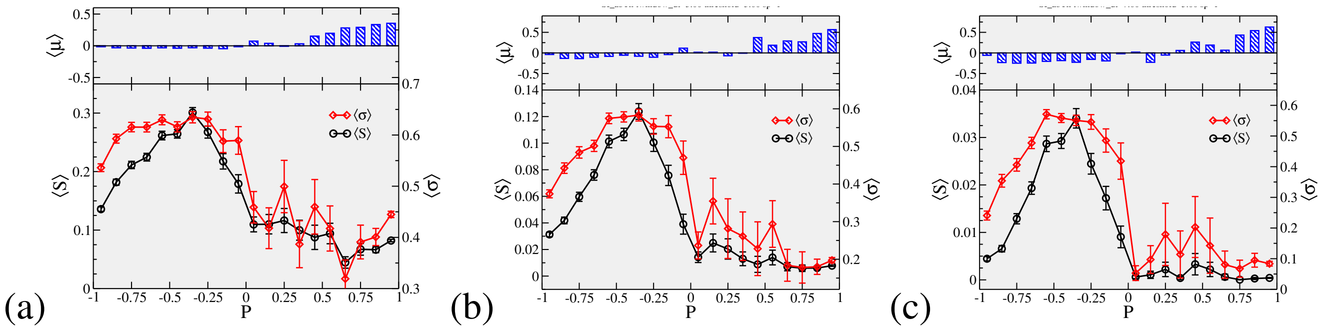


FIG. S17. Average spreadability $\langle S \rangle$ (black, left axes), diversity $\sigma$ (red, right axes), and political position $\mu$ (top panel) of the set of influence $\mathcal{I}$, as a function of the political position $P$, for the absolute-threshold model on the `20-neutral` network with (a) $\theta = 2$ days, $\Phi = 2$, (b) $\theta = 3$ days, $\Phi = 3$ and (c) $\theta = 7$ days, $\Phi = 5$. Only users with activity $a \in [10, 100]$ are considered.

TABLE S1. Some important dates and events during the impeachment process of President Dilma Rousseff, indicated by arrows in Fig. S1. The sentiment of the majority of interactions (belonging to the largest strongly connected component of the PC network, see Sec. V) collected on that day is shown in the rightmost column.

| Date | Event | Activity |
|---|---|---|
| Sun Mar 13 | Biggest street manifestation against the government spread out in more than 250 cities. | $-1$ |
| Wed Mar 16 | Supreme court permits the constitution of a commission on the chamber of deputies | $+1$ |
| Tue Mar 29 | MDB (Brazilian political party “Movimento Democrático Brasileiro”) left the government | $+1$ |
| Sun Apr 17 | Deputy chamber approves impeachment with 367 votes against 137 | $+1$ |
| Thu May 12 | Rousseff leaves the presidency after Senate approval | $-1$ |
| Mon May 23 | Audio of Senator Romero Jucá saying ”*Estancar a sangria*” | $+1$ |
| Fri Jul 29 | Rousseff delivers final arguments in the Deputy chamber | $-1$ |
| Mon Aug 29 | Rousseff’s defense in Senate | $+1$ |
| Wed Aug 31 | Senate approves impeachment with 62 to 20 votes | $+1$ |

TABLE S2. List of the 323 keywords used to collect tweets. table-keywords.pdf

| | | | | | |
|---|---|---|---|---|---|
| 13marbrasilnasruas | 13marco | 13marco2016brasilnasruas | 13marcobrasilnasruas | 13marcoeunaovou | 13marcoeuvou |
| 13marcoouvamosouelevolta | 13mareuvou | 16ago | 16agosto | 16deago | 16deagoeuvou |
| 16deagosto | 17abrilpovonasruas | 17deabril | 18marco | 18mareuvou | 31jul |
| 31juleuvou | 31julho | 31julhoavantebrasil | 31julhoconfirmado | 31julhoeuvou | 31julhopelobrasil |
| 31julvamos | 31mar | 31mareuvou | acaboudilma | acordabrasil | adeusquerida |
| aecio | aeciogolpista | aeciomedroso | aecionacadeia | aquempertenceaescola | autorizaplanejamento |
| avantetemer | bandidoviraministro | bhnasruas | bolsomito | bolsonaro | bolsonaro2018 |
| boratemer | brasilapoialavajato | brasilapoiatemer | brasilcontraogolpe | brasilcontrastf | brasilianasruas |
| brasilnasruas | brasilpaisdeladroes | brasilsempt | brazilnocorrupt | cadeia2ainstancia | caixa 2 |
| caixa2 | camara | camarasempt | censuranuncamais | cinegolpista | constituicao |
| contraogolpeedia18 | contrapec | contrapec241 | corrupcao | coxinhaco | culturapelademocracia |
| cunhagolpista | cunhanacadeia | democracia | democraciaja | deputados | derrubargolpenasruas |
| desejoprotemer | desligaogolpe | desligatv | dia13mareuvou | dia16 | dia17abril |
| dia17impeachment | dia18_03 | dia18_e_nossavez | dia18_nossavez | dia18nossavez | dia31juleuvou |
| dia31vaisermaior | dilma | dilmabandida | dilmacaixa2 | dilmacaradarenuncia | dilmaculpada |
| dilmafeiaobrasilteodeia | dilmafica | dilmaguerreira100 | dilmais | dilmajaera | dilmanaomerepresenta |
| dilmanovamente | dilmanuncamais | dilmare | diretasja | diretasja2018 | ditaduratemer |
| eduardocunhagolpe | eduardocunhagolpista | eleicoesgerais | esquentagrevegeral | estamostodoscomlula | eugritomoro |
| euquerodilmapresa | euquerolulapreso | felizaniversariomoro | ficadilma | ficalula | ficaquerida |
| ficatemer | fimdopt | forabandidos | foracomunismo | foracoxinhas | foracunha |
| foradilma | foragolpistas | foraladrao | foralula | forapt | foraserra |
| forastf | foratemer | foratemerolimpico | foratemerrio2016 | fueratemer | globogolpista |
| golpe | golpeaquinaopassa | golpeday | golpenao | golpenuncamais | golpista |
| golpistasday | grevedia29 | grevegeral | impeachment | impeachmentday | impeachmentdilma |
| impeachmentja | jantardotemer | jantartemer | jucagolpista | lavajato | lewandowskipetralha |
| libertemzedirceu | ligacaodilma | ligacaolula | lula | lula2018 | lulaacabou |
| lulacasacivil | lulacovarde | luladenunciado | lulaestamoscomvoce | lulaestamoscontigo | lulaeuconfio |
| lulaeudefendo | lulaeurespeito | lulafica | lulagolpista | lulaisworththefight | lulala |
| lulaladenovo | lulalidermundial | lulalixomundial | lulaministro | lulaministroja | lulanacadeia |
| lulanacadeiaja | lulanapapuda | lulanuncamais | lulapajaula | lulaperseguidopolitico | lulapersiste |
| lulapresidente | lulapreso | lularesiste | lulareu | lulavalealuta | lulavergonhanacional |
| lulavolta | lutarsempre | lutepelas10medidas | lutodilma | lutopelademocracia | lutopelobrasil |
| lutopt | lutosempre | mandato | marchadascoxinhas | marchadoscorruptos | marchadoscoxinhas |
| mastenhoconviccao | mblgolpista | mexeucomlulamexeucomigo | micheltemer | mobilizacaototal | moralistassemmoral |
| moropresidente | mortadeladay | mudabrasil | naoaogolpe | naovaitergolpe | naovouprarua |
| nenhumdireitoamenos | novaeleicao | novaseleicoes | obrigadompf | ocupabh | ocupabrasil |
| ocupabrasilia | ocupabrazil | ocupacopacabana | ocupaolimpiada | ocupapaulista | ocupario |
| ocuparj | ocupasaopaulo | ocupasp | ocupatudo | ocupatudocontraogolpe | ouvaiouelafica |
| ouvaiouelevolta | ouvamosouelafica | ouvamosouelevolta | ouvocevaiouelafica | panelaco | passadilma |
| pec 241 | pec 55 | pec215 | pec241 | pec55 | pecdamorte |
| pecdofimdomundo | pelademocracia | petrobras | pl2431_11 | planalto | pmdbgolpista |
| povocomlula | presaledopovo | psdb | psdbteupassadotecondena | pt | ptacabou |
| ptdesmoronando | ptexit | quedadoplanalto | quedaplanalto | queremosdilmare | renangolpista |
| renantemealavajato | renunciadadilma | renunciatemer | renunciedilma | respeiteasurnas | rippt |
| rjnasruas | saotodosgolpistas | senado | senadores | sessaodoimpeachment | simpeloimpeachment |
| somostodosgolpistas | somostodoslula | somostodosmoro | somostodospt | soscoupinbrazil | soupt |
| souptpq | souptsoudilma | souptsoulula | spnasruas | standwithlula | stf |
| stopcoupinbrazil | tchaudilmavez | tchauquerida | tchauqueridaday | teimadilma | temer |
| temereglobounidosnogolpe | temergolpista | temergolpistafrouxo | temerjamais | temermelhorquept | thauquerido |
| tocomdilma | tocomlula | todoscomdilma | todoscomlula | todosnasruas31julho | todosruadia13 |
| vaiadilma | vaiterforatemersim | vaiterimpeachment | vaiterlula | vaiterlulasim | vaiterluta |
| vaitervaia | vamostirarobrasildovermelho | vazatemer | vemprademocracia | vemprarua | vemprarua13mar |
| vemprarua17abril | vemprarua18mar | vemprarua31jul | vemprarua31julho | vempraruabrasil | voltadilma |
| voltadilmapresidenta | voltalula | voltaquerida | vomitacojantardotemer | votacaoimpeachment | |

TABLE S3. List of all the 184 hashtags classified as pro-impeachment sentiment. For each hashtag, the opinion $O_i$ of each volunteer $i$ is reported. Four choice were possible: $s = \{-1,\ 0,\ +1,\ \times\}$. table-hashtags-1.pdf

| Hashtag | $O_1$ | $O_2$ | $O_3$ | $O_4$ |
|---|---|---|---|---|
| **final classification:** −1 | | | | |
| 1 13marco2016brasilnasruas | −1 | −1 | −1 | −1 |
| 2 13mareuvou | −1 | −1 | −1 | −1 |
| 3 31julho | −1 | −1 | −1 | −1 |
| 4 31julhoconfirmado | −1 | −1 | −1 | −1 |
| 5 31julhodireitafirme | −1 | −1 | −1 | −1 |
| 6 31julhoeuvou | −1 | −1 | −1 | −1 |
| 7 31julhoforcatotal | −1 | −1 | −1 | −1 |
| 8 31julhopelobrasil | −1 | −1 | −1 | −1 |
| 9 31jullavajato | −1 | −1 | −1 | −1 |
| 10 31julvamos | −1 | −1 | −1 | −1 |
| 11 4dezvemprarua | −1 | −1 | −1 | −1 |
| 12 acaboudilma | −1 | −1 | −1 | −1 |
| 13 aceleramoro | −1 | −1 | −1 | −1 |
| 14 acelerasenado | −1 | −1 | −1 | −1 |
| 15 acelerastf | −1 | −1 | −1 | −1 |
| 16 agostotchauquerida | −1 | −1 | −1 | −1 |
| 17 antagonistasnasruas | −1 | −1 | −1 | −1 |
| 18 apoiamostemer | −1 | −1 | −1 | −1 |
| 19 aragaopetralhao | −1 | −1 | −1 | −1 |
| 20 atopelofimdopt | −1 | −1 | −1 | −1 |
| 21 avantelavajato | −1 | −1 | −1 | −1 |
| 22 avantetemer | −1 | −1 | −1 | −1 |
| 23 brasilapoiajuliomarcelo | −1 | −1 | −1 | −1 |
| 24 brasilapoiatemer | −1 | −1 | −1 | −1 |
| 25 brasillivredopt | −1 | −1 | −1 | −1 |
| 26 brasilquerlulapreso | −1 | −1 | −1 | −1 |
| 27 brasilreprovadilma | −1 | −1 | −1 | −1 |
| 28 brasilsemdilma | −1 | −1 | −1 | −1 |
| 29 brasilsempt | −1 | −1 | −1 | −1 |
| 30 brazilnocorrupt | −1 | −1 | −1 | −1 |
| 31 cadeia2ainstancia | −1 | −1 | −1 | −1 |
| 32 cadeialula | −1 | −1 | −1 | −1 |
| 33 camarasempt | −1 | −1 | −1 | −1 |
| 34 cassacaodosdireitospoliticossim | −1 | −1 | −1 | −1 |
| 35 decidamsim | −1 | −1 | −1 | −1 |
| 36 desculpasdopt | −1 | −1 | −1 | −1 |
| 37 dia13mareuvou | −1 | −1 | −1 | −1 |
| 38 dia31juleuvou | −1 | −1 | −1 | −1 |
| 39 dilmabandida | −1 | −1 | −1 | −1 |
| 40 dilmacaixa2 | −1 | −1 | −1 | −1 |
| 41 dilmaculpada | −1 | −1 | −1 | −1 |
| 42 dilmaculpadaoea | −1 | −1 | −1 | −1 |
| 43 dilmafungo | −1 | −1 | −1 | −1 |
| 44 dilmagolpista | −1 | −1 | −1 | −1 |
| 45 dilmajaera | −1 | −1 | −1 | −1 |
| 46 dilmamente | −1 | −1 | −1 | −1 |
| 47 dilmamentirosa | −1 | −1 | −1 | −1 |
| 48 dilmanacadeia | −1 | −1 | −1 | −1 |
| 49 dilmanaomerepresenta | −1 | −1 | −1 | −1 |
| 50 dilmare | −1 | −1 | −1 | −1 |
| 51 euapoiodeltan | −1 | −1 | −1 | −1 |
| 52 eugritomoro | −1 | −1 | −1 | −1 |
| 53 eulutopelomoro | −1 | −1 | −1 | −1 |
| 54 euquerolulapreso | −1 | −1 | −1 | −1 |
| 55 eusoumoro | −1 | −1 | −1 | −1 |
| 56 extincaodopt | −1 | −1 | −1 | −1 |
| 57 ficatemer | −1 | −1 | −1 | −1 |
| 58 fimdopt | −1 | −1 | −1 | −1 |
| 59 foracomunismo | −1 | −1 | −1 | −1 |
| 60 foradilma | −1 | −1 | −1 | −1 |
| 61 foradilmalula | −1 | −1 | −1 | −1 |
| 62 foralula | −1 | −1 | −1 | −1 |
| 63 forapt | −1 | −1 | −1 | −1 |
| 64 herancamaldita | −1 | −1 | −1 | −1 |
| 65 impeachmentdilmaja | −1 | −1 | −1 | −1 |
| 66 impeachmentsim | −1 | −1 | −1 | −1 |
| 67 independenciasempt | −1 | −1 | −1 | −1 |
| 68 lavajato | −1 | −1 | −1 | −1 |
| 69 lavajatoeuapoio | −1 | −1 | −1 | −1 |
| 70 lulacovarde | −1 | −1 | −1 | −1 |
| 71 luladenunciado | −1 | −1 | −1 | −1 |
| 72 luladenunciadonalavajato | −1 | −1 | −1 | −1 |
| 73 lulaedilmanacadeia | −1 | −1 | −1 | −1 |
| 74 lulagolpista | −1 | −1 | −1 | −1 |
| 75 lulaladrao | −1 | −1 | −1 | −1 |
| 76 lulalixomundial | −1 | −1 | −1 | −1 |
| 77 lulamente | −1 | −1 | −1 | −1 |
| 78 lulanacadeia | −1 | −1 | −1 | −1 |
| 79 lulanacadeiaja | −1 | −1 | −1 | −1 |
| 80 lulanuncamais | −1 | −1 | −1 | −1 |
| 81 lulapajaula | −1 | −1 | −1 | −1 |
| 82 lulapresoja | −1 | −1 | −1 | −1 |
| 83 lulareu | −1 | −1 | −1 | −1 |
| 84 lulavaipromoro | −1 | −1 | −1 | −1 |
| 85 lulavergonhanacional | −1 | −1 | −1 | −1 |
| 86 maranhaoempregadodopt | −1 | −1 | −1 | −1 |
| 87 mexeucommoromexeucomigo | −1 | −1 | −1 | −1 |
| 88 morobrasilteapoia | −1 | −1 | −1 | −1 |
| 89 morolidermundial | −1 | −1 | −1 | −1 |
| 90 moropresidente | −1 | −1 | −1 | −1 |
| 91 novaseleicoesnao | −1 | −1 | −1 | −1 |
| 92 oabdopt | −1 | −1 | −1 | −1 |
| 93 oabrepete92 | −1 | −1 | −1 | −1 |
| 94 obrigadampf | −1 | −1 | −1 | −1 |
| 95 obrigadompf | −1 | −1 | −1 | −1 |
| 96 ocupabh | −1 | −1 | −1 | −1 |
| 97 olimpiadassemdilma | −1 | −1 | −1 | −1 |
| 98 ouvocevaiouelafica | −1 | −1 | −1 | −1 |
| 99 passadilma | −1 | −1 | −1 | −1 |
| 100 prendehojemoro | −1 | −1 | −1 | −1 |
| 101 ptacabou | −1 | −1 | −1 | −1 |
| 102 ptdesmoronando | −1 | −1 | −1 | −1 |
| 103 ptexit | −1 | −1 | −1 | −1 |
| 104 ptnuncamais | −1 | −1 | −1 | −1 |
| 105 ptraidoresdobrasil | −1 | −1 | −1 | −1 |
| 106 ptvergonhanacional | −1 | −1 | −1 | −1 |
| 107 quedadoplanalto | −1 | −1 | −1 | −1 |
| 108 quedaplanalto | −1 | −1 | −1 | −1 |
| 109 renunciadilma | −1 | −1 | −1 | −1 |
| 110 renunciedilma | −1 | −1 | −1 | −1 |
| 111 repudionomeacaolula | −1 | −1 | −1 | −1 |
| 112 senadovotesim | −1 | −1 | −1 | −1 |
| 113 setembrosemdilma | −1 | −1 | −1 | −1 |
| 114 simpeloimpeachment | −1 | −1 | −1 | −1 |
| 115 somosmoro | −1 | −1 | −1 | −1 |
| 116 somostodosjanaina | −1 | −1 | −1 | −1 |
| 117 somostodosmoro | −1 | −1 | −1 | −1 |
| 118 soumoro | −1 | −1 | −1 | −1 |
| 119 tchaumaldita | −1 | −1 | −1 | −1 |
| 120 tchaupt | −1 | −1 | −1 | −1 |
| 121 tchauquerida | −1 | −1 | −1 | −1 |
| 122 tchauqueridaday | −1 | −1 | −1 | −1 |
| 123 temermelhorquept | −1 | −1 | −1 | −1 |
| 124 todoapoioalavajato | −1 | −1 | −1 | −1 |
| 125 todoscontratoffoli | −1 | −1 | −1 | −1 |
| 126 todosnasruas31julho | −1 | −1 | −1 | −1 |
| 127 ultimopanelaco | −1 | −1 | −1 | −1 |
| 128 vaiadilma | −1 | −1 | −1 | −1 |
| 129 vaiterimpeachment | −1 | −1 | −1 | −1 |
| 130 vamostirarobrasildovermelho | −1 | −1 | −1 | −1 |
| 131 vazavacaloca | −1 | −1 | −1 | −1 |
| 132 vempelomoro | −1 | −1 | −1 | −1 |
| 133 vempradetencao | −1 | −1 | −1 | −1 |
| 134 vemprafiesp | −1 | −1 | −1 | −1 |
| 135 vemprarua13mar | −1 | −1 | −1 | −1 |
| 136 vemprarua13marco | −1 | −1 | −1 | −1 |
| 137 vemprarua17abril | −1 | −1 | −1 | −1 |
| 138 vemprarua31jul | −1 | −1 | −1 | −1 |
| 139 vemprarua31julho | −1 | −1 | −1 | −1 |
| **final classification:** −1* | | | | |
| 1 04dezvemprarua | −1 | −1 | −1 | × |
| 2 13marco | −1 | × | −1 | −1 |
| 3 13marcoeuvou | −1 | −1 | +1 | −1 |
| 4 31juleuvou | −1 | −1 | +1 | −1 |
| 5 31julhoavantebrasil | × | −1 | −1 | −1 |
| 6 4dezeuvou | × | −1 | −1 | −1 |
| 7 avantepf | −1 | −1 | −1 | 0 |
| 8 boratemer | −1 | −1 | −1 | 0 |
| 9 brasilapoialavajato | −1 | −1 | −1 | × |
| 10 brasilnasruas | −1 | −1 | −1 | × |
| 11 brasilnasruas20nov | −1 | −1 | −1 | × |
| 12 crimeabandeirabr | −1 | −1 | −1 | +1 |
| 13 deolhonostf | −1 | −1 | −1 | +1 |
| 14 dilmanuncamais | −1 | −1 | +1 | −1 |
| 15 felizaniversariomoro | −1 | −1 | −1 | × |
| 16 impeachj | −1 | × | −1 | −1 |
| 17 impeachmentdilma | −1 | 0 | −1 | −1 |
| 18 juntospelalavajato | −1 | −1 | −1 | 0 |
| 19 lavajatopatrimoniodopovo | −1 | −1 | −1 | × |
| 20 lewandowskigolpista | −1 | −1 | −1 | +1 |
| 21 lewandowskipetralha | −1 | −1 | −1 | 0 |
| 22 liberadelacaojanot | −1 | −1 | 0 | −1 |
| 23 lulaacabou | −1 | −1 | −1 | 0 |
| 24 luladrao | +1 | −1 | −1 | −1 |
| 25 lulanapapuda | −1 | −1 | −1 | +1 |
| 26 lulapreso | −1 | −1 | −1 | 0 |
| 27 mortadeladay | +1 | −1 | −1 | −1 |
| 28 naomexanalavajato | −1 | −1 | −1 | × |
| 29 nasruas15nov | × | −1 | −1 | −1 |
| 30 novaeleicaoehgolpe | −1 | −1 | +1 | −1 |
| 31 novogoverno | −1 | −1 | −1 | 0 |
| 32 ocupasaopaulo | −1 | 0 | −1 | −1 |
| 33 orgulhodapf | −1 | −1 | −1 | × |
| 34 petrolao | × | −1 | −1 | −1 |
| 35 propinocracia | 0 | −1 | −1 | −1 |
| 36 queremosdilmare | −1 | −1 | −1 | +1 |
| 37 renannacadeia | 0 | −1 | −1 | −1 |
| 38 somostodosdeltan | −1 | −1 | −1 | × |
| 39 somostodosvallisney | −1 | −1 | −1 | × |
| 40 stfretrocessonao | −1 | −1 | −1 | × |
| 41 tchaudilmavez | −1 | −1 | −1 | +1 |
| 42 temereouro | −1 | −1 | −1 | 0 |
| 43 teoricorrupto | −1 | −1 | −1 | +1 |
| 44 teoridevolveolula | +1 | −1 | −1 | −1 |
| 45 vempraruabrasil | 0 | −1 | −1 | −1 |

TABLE S4. List of all the 200 hashtags classified as anti-impeachment sentiment. For each hashtag, the opinion $O_i$ of each volunteer $i$ is reported. Four choice were possible: $s = \{-1,\ 0,\ +1,\ \times\}$. table-hashtags-2.pdf

| Hashtag | $O_1$ | $O_2$ | $O_3$ | $O_4$ |
|---|---|---|---|---|
| **final classification:** +1 | | | | |
| 1 180diasdegolpe | +1 | +1 | +1 | +1 |
| 2 54milhoesdedilmas | +1 | +1 | +1 | +1 |
| 3 acaradogolpe | +1 | +1 | +1 | +1 |
| 4 aeciogolpista | +1 | +1 | +1 | +1 |
| 5 agoraerua | +1 | +1 | +1 | +1 |
| 6 alutacomecou | +1 | +1 | +1 | +1 |
| 7 amarsemtemer | +1 | +1 | +1 | +1 |
| 8 anulamaranhao | +1 | +1 | +1 | +1 |
| 9 anulastf | +1 | +1 | +1 | +1 |
| 10 anulatudosupremo | +1 | +1 | +1 | +1 |
| 11 apoioalula | +1 | +1 | +1 | +1 |
| 12 avantetemerpracadeia | +1 | +1 | +1 | +1 |
| 13 baralhodogolpe | +1 | +1 | +1 | +1 |
| 14 barulhacoforatemer | +1 | +1 | +1 | +1 |
| 15 blogueiroscomdilma | +1 | +1 | +1 | +1 |
| 16 brasilcontraogolpe | +1 | +1 | +1 | +1 |
| 17 byedemocracyday | +1 | +1 | +1 | +1 |
| 18 cinegolpista | +1 | +1 | +1 | +1 |
| 19 comlulaporlula | +1 | +1 | +1 | +1 |
| 20 coupinbrazil | +1 | +1 | +1 | +1 |
| 21 culturapeladecmocracia | +1 | +1 | +1 | +1 |
| 22 cunhagolpista | +1 | +1 | +1 | +1 |
| 23 decidapelademocracia | +1 | +1 | +1 | +1 |
| 24 derrubargolpenasruas | +1 | +1 | +1 | +1 |
| 25 devolverenan | +1 | +1 | +1 | +1 |
| 26 dia31vaisermaior | +1 | +1 | +1 | +1 |
| 27 dilmacoracaovalente | +1 | +1 | +1 | +1 |
| 28 dilmaeinocente | +1 | +1 | +1 | +1 |
| 29 dilmafica | +1 | +1 | +1 | +1 |
| 30 dilmaficagolpesai | +1 | +1 | +1 | +1 |
| 31 dilmanatvbrasil | +1 | +1 | +1 | +1 |
| 32 dilmavolta | +1 | +1 | +1 | +1 |
| 33 diretasja | +1 | +1 | +1 | +1 |
| 34 ditaduratemer | +1 | +1 | +1 | +1 |
| 35 eduardocunhagolpista | +1 | +1 | +1 | +1 |
| 36 egolpe | +1 | +1 | +1 | +1 |
| 37 egolpesim | +1 | +1 | +1 | +1 |
| 38 elmundocondilma | +1 | +1 | +1 | +1 |
| 39 emdefesadademocracia | +1 | +1 | +1 | +1 |
| 40 entrouparaolixodahistoria | +1 | +1 | +1 | +1 |
| 41 esquentagrevegeral | +1 | +1 | +1 | +1 |
| 42 estamoscomlula | +1 | +1 | +1 | +1 |
| 43 estamostodoscomlula | +1 | +1 | +1 | +1 |
| 44 estoucomlula | +1 | +1 | +1 | +1 |
| 45 fairplayparadilma | +1 | +1 | +1 | +1 |
| 46 ficadilma | +1 | +1 | +1 | +1 |
| 47 foracoxinhas | +1 | +1 | +1 | +1 |
| 48 foragilmar | +1 | +1 | +1 | +1 |
| 49 foragolpista | +1 | +1 | +1 | +1 |
| 50 foragolpistas | +1 | +1 | +1 | +1 |
| 51 foratemerficahaddad | +1 | +1 | +1 | +1 |
| 52 foratemergolpista | +1 | +1 | +1 | +1 |
| 53 foratemerladrao | +1 | +1 | +1 | +1 |
| 54 foratemerolimpico | +1 | +1 | +1 | +1 |
| 55 foratemerrio2016 | +1 | +1 | +1 | +1 |
| 56 forcadilma | +1 | +1 | +1 | +1 |
| 57 forcalula | +1 | +1 | +1 | +1 |
| 58 forcaquerida | +1 | +1 | +1 | +1 |
| 59 getouttemer | +1 | +1 | +1 | +1 |
| 60 globogolpista | +1 | +1 | +1 | +1 |
| 61 golpeaquinaopassa | +1 | +1 | +1 | +1 |
| 62 golpeday | +1 | +1 | +1 | +1 |
| 63 golpedeestado | +1 | +1 | +1 | +1 |
| 64 golpeemachista | +1 | +1 | +1 | +1 |
| 65 golpenao | +1 | +1 | +1 | +1 |
| 66 golpenuncamais | +1 | +1 | +1 | +1 |
| 67 golpismodamidia | +1 | +1 | +1 | +1 |
| 68 golpista | +1 | +1 | +1 | +1 |
| 69 golpistas | +1 | +1 | +1 | +1 |
| 70 golpistasday | +1 | +1 | +1 | +1 |
| 71 gritocontraogolpe | +1 | +1 | +1 | +1 |
| 72 gritodosexcluidos | +1 | +1 | +1 | +1 |
| 73 impeachmentsemcrimeegolpe | +1 | +1 | +1 | +1 |
| 74 jatemluta | +1 | +1 | +1 | +1 |
| 75 jucagolpista | +1 | +1 | +1 | +1 |
| 76 lulaestamoscomvoce | +1 | +1 | +1 | +1 |
| 77 lulaestamoscontigo | +1 | +1 | +1 | +1 |
| 78 lulaeterno | +1 | +1 | +1 | +1 |
| 79 lulaeuconfio | +1 | +1 | +1 | +1 |
| 80 lulaeudefendo | +1 | +1 | +1 | +1 |
| 81 lulaeurespeito | +1 | +1 | +1 | +1 |
| 82 lulafica | +1 | +1 | +1 | +1 |
| 83 lulaisworththefight | +1 | +1 | +1 | +1 |
| 84 lulalidermundial | +1 | +1 | +1 | +1 |
| 85 lulaministroja | +1 | +1 | +1 | +1 |
| 86 lulaperseguidopolitico | +1 | +1 | +1 | +1 |
| 87 lulapresidente | +1 | +1 | +1 | +1 |
| 88 lulario2016 | +1 | +1 | +1 | +1 |
| 89 lulavalealuta | +1 | +1 | +1 | +1 |
| 90 lulavolta | +1 | +1 | +1 | +1 |
| 91 lutapelademocracia | +1 | +1 | +1 | +1 |
| 92 lutarsempre | +1 | +1 | +1 | +1 |
| 93 lutopelademocracia | +1 | +1 | +1 | +1 |
| 94 marchadascoxinhas | +1 | +1 | +1 | +1 |
| 95 marchadoscorruptos | +1 | +1 | +1 | +1 |
| 96 marchadoscoxinhas | +1 | +1 | +1 | +1 |
| 97 marchadospatinhospamonhas | +1 | +1 | +1 | +1 |
| 98 mblgolpista | +1 | +1 | +1 | +1 |
| 99 mentiraenaglobo | +1 | +1 | +1 | +1 |
| 100 mexeucomlulamexeucomigo | +1 | +1 | +1 | +1 |
| 101 mobilizacaototal | +1 | +1 | +1 | +1 |
| 102 moralistassemmoral | +1 | +1 | +1 | +1 |
| 103 moroamigodecunha | +1 | +1 | +1 | +1 |
| 104 moroexonerado | +1 | +1 | +1 | +1 |
| 105 moronacadeia | +1 | +1 | +1 | +1 |
| 106 mulherescontratemer | +1 | +1 | +1 | +1 |
| 107 naoaogolpe | +1 | +1 | +1 | +1 |
| 108 naovaitergolpe | +1 | +1 | +1 | +1 |
| 109 naovoupagaropacto | +1 | +1 | +1 | +1 |
| 110 ocupaminc | +1 | +1 | +1 | +1 |
| 111 ocupaolimpiada | +1 | +1 | +1 | +1 |
| 112 ocuparedeesgoto | +1 | +1 | +1 | +1 |
| 113 ocupasenado | +1 | +1 | +1 | +1 |
| 114 ocupatudo | +1 | +1 | +1 | +1 |
| 115 ocupatudocontraogolpe | +1 | +1 | +1 | +1 |
| 116 ogolpeefichasuja | +1 | +1 | +1 | +1 |
| 117 opovodecide | +1 | +1 | +1 | +1 |
| 118 opovoquerdemocracia | +1 | +1 | +1 | +1 |
| 119 parabenspresidentadilma | +1 | +1 | +1 | +1 |
| 120 pelademocracia | +1 | +1 | +1 | +1 |
| 121 pmdbgolpista | +1 | +1 | +1 | +1 |
| 122 povocomlula | +1 | +1 | +1 | +1 |
| 123 psdbteupassadotecondena | +1 | +1 | +1 | +1 |
| 124 queremcalaraune | +1 | +1 | +1 | +1 |
| 125 ralatemer | +1 | +1 | +1 | +1 |
| 126 reformanaorenunciasim | +1 | +1 | +1 | +1 |
| 127 renangolpista | +1 | +1 | +1 | +1 |
| 128 renunciatemer | +1 | +1 | +1 | +1 |
| 129 respeiteasurnas | +1 | +1 | +1 | +1 |
| 130 ripdemocracia | +1 | +1 | +1 | +1 |
| 131 semdemocraciasempaz | +1 | +1 | +1 | +1 |
| 132 senadovotenao | +1 | +1 | +1 | +1 |
| 133 somostodoslula | +1 | +1 | +1 | +1 |
| 134 somostodospt | +1 | +1 | +1 | +1 |
| 135 soscoupinbrazil | +1 | +1 | +1 | +1 |
| 136 soupelademocracia | +1 | +1 | +1 | +1 |
| 137 soupt | +1 | +1 | +1 | +1 |
| 138 standwhitlula | +1 | +1 | +1 | +1 |
| 139 standwithlula | +1 | +1 | +1 | +1 |
| 140 stopcoupinbrazil | +1 | +1 | +1 | +1 |
| 141 teimadilma | +1 | +1 | +1 | +1 |
| 142 temercaradepau | +1 | +1 | +1 | +1 |
| 143 temerecunha | +1 | +1 | +1 | +1 |
| 144 temereglobounidosnogolpe | +1 | +1 | +1 | +1 |
| 145 temergolpista | +1 | +1 | +1 | +1 |
| 146 temergolpistafrouxo | +1 | +1 | +1 | +1 |
| 147 temerjamais | +1 | +1 | +1 | +1 |
| 148 temerout | +1 | +1 | +1 | +1 |
| 149 tocomdilma | +1 | +1 | +1 | +1 |
| 150 tocomlula | +1 | +1 | +1 | +1 |
| 151 todoscomdilma | +1 | +1 | +1 | +1 |
| 152 todoscomlula | +1 | +1 | +1 | +1 |
| 153 tonaruaforatemer | +1 | +1 | +1 | +1 |
| 154 vaiterforatemersim | +1 | +1 | +1 | +1 |
| 155 vaiterlula | +1 | +1 | +1 | +1 |
| 156 vaiterluta | +1 | +1 | +1 | +1 |
| 157 vamosbarrarosgolpistas | +1 | +1 | +1 | +1 |
| 158 vempademocracia | +1 | +1 | +1 | +1 |
| 159 volta_querida_democracia | +1 | +1 | +1 | +1 |
| 160 voltadilma | +1 | +1 | +1 | +1 |
| 161 voltadilmapresidenta | +1 | +1 | +1 | +1 |
| 162 voltalula | +1 | +1 | +1 | +1 |
| 163 voltaquerida | +1 | +1 | +1 | +1 |
| **final classification:** +1* | | | | |
| 1 anulateori | +1 | +1 | +1 | 0 |
| 2 brasiljusto | −1 | +1 | +1 | +1 |
| 3 censuranuncamais | +1 | +1 | × | +1 |
| 4 coxinhaco | −1 | +1 | +1 | +1 |
| 5 cunhaetemer | × | +1 | +1 | +1 |
| 6 cunhanacadeia | +1 | +1 | 0 | +1 |
| 7 cunhasnacadeia | 0 | +1 | +1 | +1 |
| 8 democraciaja | × | +1 | +1 | +1 |
| 9 desapegadolulastf | +1 | +1 | −1 | +1 |
| 10 desligaogolpe | × | +1 | +1 | +1 |
| 11 desligatv | +1 | × | +1 | +1 |
| 12 dilmanovamente | +1 | 0 | +1 | +1 |
| 13 eleicaoja | 0 | +1 | +1 | +1 |
| 14 eleicoesja | +1 | 0 | +1 | +1 |
| 15 ficalula | −1 | +1 | +1 | +1 |
| 16 ficaquerida | +1 | +1 | +1 | 0 |
| 17 foraserra | 0 | +1 | +1 | +1 |
| 18 fueratemer | +1 | +1 | 0 | +1 |
| 19 golpe | +1 | +1 | × | +1 |
| 20 grevegeral | +1 | × | +1 | +1 |
| 21 joaopaulo13comlula | × | +1 | +1 | +1 |
| 22 libertemzedirceu | +1 | × | +1 | +1 |
| 23 lula2018 | +1 | 0 | +1 | +1 |
| 24 lulacasacivil | +1 | +1 | +1 | 0 |
| 25 lulaladenovo | +1 | 0 | +1 | +1 |
| 26 lularesiste | −1 | +1 | +1 | +1 |
| 27 lutareumdireito | +1 | +1 | −1 | +1 |
| 28 naotemarrego | +1 | × | +1 | +1 |
| 29 natalsemtemer | 0 | +1 | +1 | +1 |
| 30 nenhumdireitoamenos | +1 | +1 | +1 | 0 |
| 31 ocupabrasilia | +1 | +1 | −1 | +1 |
| 32 renunciacunha | 0 | +1 | +1 | +1 |
| 33 stfacovardado | +1 | 0 | +1 | +1 |
| 34 temersilveriodosreis | +1 | −1 | +1 | +1 |
| 35 traidoresdopovo | +1 | +1 | −1 | +1 |
| 36 vaitervaia | +1 | +1 | −1 | +1 |
| 37 vazatemer | 0 | +1 | +1 | +1 |

TABLE S5. List of all the 20 hashtags classified as neutral sentiment ($s = 0$) and all the 39 hashtags classified as not related ($s = \times$). For each hashtag, the opinion $O_i$ of each volunteer $i$ is reported. Four choice were possible: $s = \{-1,\ 0,\ +1,\ \times\}$. table-hashtags-3.pdf

| Hashtag | $O_1$ | $O_2$ | $O_3$ | $O_4$ |
|---|---|---|---|---|
| **final classification:** 0 | | | | |
| 1 foracorruptos | 0 | 0 | 0 | 0 |
| 2 impeachment | 0 | 0 | 0 | 0 |
| 3 tchaucunha | 0 | 0 | 0 | 0 |
| **final classification:** $0^*$ | | | | |
| 1 delatacunha | 0 | +1 | 0 | 0 |
| 2 dilma | −1 | 0 | 0 | 0 |
| 3 dilmanosbt | +1 | 0 | 0 | 0 |
| 4 dilmarousseff | 0 | 0 | 0 | −1 |
| 5 diretasja2018 | 0 | 0 | −1 | 0 |
| 6 eduardocunha | 0 | 0 | × | 0 |
| 7 ficamedina | × | 0 | 0 | 0 |
| 8 forabandidos | 0 | 0 | −1 | 0 |
| 9 foraminc | 0 | 0 | 0 | +1 |
| 10 forastf | 0 | 0 | 0 | −1 |
| 11 foratodosratos | 0 | 0 | × | 0 |
| 12 janotgolpista | 0 | 0 | 0 | −1 |
| 13 seeufosseadilma | −1 | 0 | 0 | 0 |
| 14 sessaodoimpeachment | −1 | 0 | 0 | 0 |
| 15 stfvergonhanacional | 0 | 0 | 0 | × |
| 16 vemprarua | 0 | 0 | 0 | −1 |
| 17 votacaoimpeachment | −1 | 0 | 0 | 0 |

| Hashtag | $O_1$ | $O_2$ | $O_3$ | $O_4$ |
|---|---|---|---|---|
| **final classification:** × | | | | |
| 1 16ago | × | × | × | × |
| 2 18marco | × | × | × | × |
| 3 brasilnaonu | × | × | × | × |
| 4 camara | × | × | × | × |
| 5 constituicao | × | × | × | × |
| 6 dia18 | × | × | × | × |
| 7 dia18_03 | × | × | × | × |
| 8 golacosdadilma | × | × | × | × |
| 9 justica | × | × | × | × |
| 10 listatripliceagu | × | × | × | × |
| 11 mandato | × | × | × | × |
| 12 moroaguarda | × | × | × | × |
| 13 mpf | × | × | × | × |
| 14 ocupabrazil | × | × | × | × |
| 15 senadores | × | × | × | × |
| 16 timepetrobras | × | × | × | × |
| **final classification:** $\times^*$ | | | | |
| 1 10medidassemgolpe | × | × | × | 0 |
| 2 31mar | × | × | × | +1 |
| 3 anistiacaixa2nao | × | × | 0 | × |
| 4 anistiarcaixa2egolpe | × | × | 0 | × |
| 5 bolsonaro | × | × | −1 | × |
| 6 bolsonaro2018 | × | × | −1 | × |
| 7 bolsonaropresidente | × | × | −1 | × |
| 8 contraogolpeedia18 | × | +1 | × | × |
| 9 corrupcao | 0 | × | × | × |
| 10 cunha | × | × | × | 0 |
| 11 delcidiotemrazao | × | × | × | −1 |
| 12 deputados | × | × | × | 0 |
| 13 dilmacaradarenuncia | × | +1 | × | × |
| 14 eleicoes2016 | × | × | 0 | × |
| 15 listafechadanao | × | × | 0 | × |
| 16 martraira | × | × | × | −1 |
| 17 ocupario | × | × | −1 | × |
| 18 petrobras | 0 | × | × | × |
| 19 planalto | × | × | × | 0 |
| 20 politica | +1 | × | × | × |
| 21 presaledopovo | +1 | × | × | × |
| 22 senado | +1 | × | × | × |
| 23 stf | × | × | × | 0 |

TABLE S6. Final number of hashtags for each category. The symbols in superscript between parenthesis correspond to the ones used in Tables S3 to S5 and main text. Three different levels of agreement are listed: full agreement (full); 3/4 agreement (partial); and less than 3 agreements (divergent). In the modified classification, we include the 52 hashtags with divergent classification in the neutral class, see text.

| | full | partial ($^*$) | divergent ($^?$) | total |
|---|---|---|---|---|
| −1 | 139 | 45 | — | 184 |
| 0 | 3 | 17 | 0 (52) | 20 (72) |
| +1 | 163 | 37 | — | 200 |
| × | 16 | 23 | 52 (0) | 91 (39) |
| total | 321 | 122 | 52 | 495 |

TABLE S7. List of the 52 hashtags for which an agreement was not achieved. For each hashtag, the opinion $O_i$ of each volunteer $i$ is reported. Four choice were possible: $s = \{-1,\ 0,\ +1,\ \times\}$. table-divergent.pdf

| Hashtag | $O_1$ | $O_2$ | $O_3$ | $O_4$ |
|---|---|---|---|---|
| **final classification:** $0^?$ | | | | |
| 1 2ainstanciacadeia | $\times$ | $-1$ | $-1$ | $\times$ |
| 2 aceleralavajatostf | $\times$ | $\times$ | $-1$ | $-1$ |
| 3 acordabrasil | $-1$ | 0 | $-1$ | $\times$ |
| 4 adeuscunha | $\times$ | $+1$ | 0 | $+1$ |
| 5 brasilcontrastf | $-1$ | $+1$ | 0 | $\times$ |
| 6 comandantelula | $\times$ | 0 | 0 | $-1$ |
| 7 cunhacaiu | $-1$ | 0 | $+1$ | $+1$ |
| 8 desejoprotemer | $+1$ | $-1$ | 0 | 0 |
| 9 eavezdasmulheres | $\times$ | $\times$ | $+1$ | $+1$ |
| 10 fimforoprivilegiado | 0 | 0 | $\times$ | $\times$ |
| 11 foracunha | $-1$ | $+1$ | $+1$ | 0 |
| 12 forajuca | 0 | $+1$ | $+1$ | $-1$ |
| 13 foraladrao | 0 | $-1$ | $\times$ | $+1$ |
| 14 foraoab | $\times$ | $\times$ | $+1$ | $+1$ |
| 15 forapmdb | 0 | 0 | $+1$ | $+1$ |
| 16 forarenan | $\times$ | 0 | $+1$ | $+1$ |
| 17 forarodrigomaia | 0 | $-1$ | 0 | $+1$ |
| 18 foratemer | $+1$ | 0 | 0 | $+1$ |
| 19 foratodos | 0 | $+1$ | 0 | $\times$ |
| 20 impeachmentbrazil | $-1$ | 0 | 0 | $+1$ |
| 21 impeachmentday | $-1$ | 0 | $+1$ | 0 |
| 22 impeachmentja | $\times$ | $-1$ | $-1$ | 0 |
| 23 jucanacadeia | $+1$ | $+1$ | 0 | 0 |
| 24 lula | $+1$ | 0 | $\times$ | 0 |
| 25 lulala | $-1$ | $\times$ | $-1$ | $+1$ |
| 26 lulaministro | $+1$ | 0 | 0 | $+1$ |
| 27 lulanorecife | $+1$ | 0 | 0 | $\times$ |
| 28 mapadoimpeachment | $-1$ | 0 | $-1$ | 0 |
| 29 mastenhoconviccao | $\times$ | 0 | $+1$ | $+1$ |
| 30 micheltemer | $\times$ | 0 | $\times$ | 0 |
| 31 mudabrasil | $-1$ | 0 | $\times$ | 0 |
| 32 ocupabrasil | 0 | $+1$ | $-1$ | 0 |
| 33 ocupacopacabana | $\times$ | 0 | $+1$ | $+1$ |
| 34 ocupapaulista | $-1$ | $+1$ | $-1$ | 0 |
| 35 ocuparj | $-1$ | $\times$ | $+1$ | $\times$ |
| 36 ocupasp | $-1$ | 0 | $-1$ | $\times$ |
| 37 ocupastf | $+1$ | 0 | 0 | $+1$ |
| 38 olimpeachment | $+1$ | $-1$ | $-1$ | 0 |
| 39 panelaco | $\times$ | $\times$ | $-1$ | $+1$ |
| 40 possedadesonra | $\times$ | $+1$ | $+1$ | 0 |
| 41 renanpreso | 0 | $\times$ | 0 | $\times$ |
| 42 renanreu | $\times$ | $-1$ | 0 | $\times$ |
| 43 renantemealavajato | $-1$ | $-1$ | 0 | $\times$ |
| 44 renunciaja | 0 | $-1$ | $-1$ | $+1$ |
| 45 salvealavajato | $\times$ | $-1$ | $-1$ | $\times$ |
| 46 sergiomoro | $-1$ | 0 | $-1$ | 0 |
| 47 somostodosgolpistas | $-1$ | $-1$ | $+1$ | $+1$ |
| 48 souptpq | $\times$ | $+1$ | $+1$ | 0 |
| 49 tchauquerido | $\times$ | $+1$ | $-1$ | $\times$ |
| 50 temer | $\times$ | 0 | $\times$ | 0 |
| 51 teorigolpista | $-1$ | $\times$ | $+1$ | $+1$ |
| 52 vergonhacongressobr | $\times$ | $+1$ | $+1$ | $\times$ |

TABLE S8. Properties of the `20-neutral`, `72-neutral` integrated networks considering the SCC (top) and whole network (bottom). $N$ is the total number of nodes; $L$ is the number of links; $\langle k_{\text{out}}^n \rangle$ is the $n$-th moment of the number of links; $E$ is the number of interactions; $\langle a^n \rangle$ is the $n$-th moment of the activity. The average weight of the links is denoted by $\langle W_{ij} \rangle$; $N_+$ and $N_-$ are the numbers of nodes with overall anti- and pro-impeachment position, respectively.

**Largest strongly connected component:**

| | $N$ | $L$ | $\langle k_{\text{out}} \rangle$ | $\langle k_{\text{out}}^2 \rangle$ | $W$ | $\langle a \rangle$ | $\langle a^2 \rangle$ | $\langle W_{ij} \rangle$ | $N_+$ | $N_-$ | $Q$ |
|---|---|---|---|---|---|---|---|---|---|---|---|
| `20-neutral` | 31 412 | 833 123 | 26.52 | 4 727.82 | 1 552 389 | 49.42 | 44 162.64 | 1.86 | 13925 | 16257 | 0.435 |
| `72-neutral` | 39 525 | 1 063 699 | 26.91 | 5 251.52 | 2 056 448 | 52.03 | 50 110.90 | 1.93 | 16352 | 18340 | 0.431 |

**Whole network:**

| | $N$ | $L$ | $\langle k_{\text{out}} \rangle$ | $\langle k_{\text{out}}^2 \rangle$ | $W$ | $\langle a \rangle$ | $\langle a^2 \rangle$ | $\langle W_{ij} \rangle$ | $N_+$ | $N_-$ | $Q$ |
|---|---|---|---|---|---|---|---|---|---|---|---|
| `20-neutral` | 285 670 | 1 696 841 | 5.94 | 818.25 | 2 722 504 | 9.53 | 8 242.83 | 1.60 | 101 250 | 125 591 | — |
| `72-neutral` | 437 728 | 2 341 473 | 5.35 | 768.02 | 3 759 684 | 8.59 | 7 404.21 | 1.61 | 101 250 | 125 591 | — |

TABLE S9. Community structure of the networks `20-neutral` and `72-neutral`, according to the Louvain algorithm.Very small communities with only a few nodes are omitted due to the resolution limit of the modularity optimization [17].

| `20-neutral` | | `72-neutral` | |
|---|---|---|---|
| Size | $\langle P \rangle$ | Size | $\langle P \rangle$ |
| 10502 | $0.840 \pm 0.437$ | 12570 | $0.598 \pm 0.438$ |
| 9937 | $-0.687 \pm 0.428$ | 11821 | $-0.566 \pm 0.436$ |
| 4238 | $-0.097 \pm 0.852$ | 6489 | $-0.009 \pm 0.654$ |
| 3708 | $-0.011 \pm 0.829$ | 5531 | $-0.045 \pm 0.698$ |
| 2599 | $-0.529 \pm 0.427$ | 2711 | $-0.481 \pm 0.393$ |
| 170 | $-0.484 \pm 0.781$ | 254 | $-0.217 \pm 0.764$ |
| 52 | $-0.043 \pm 0.884$ | 23 | $-0.433 \pm 0.592$ |
| 37 | $-0.448 \pm 0.696$ | 19 | $-0.863 \pm 0.217$ |
| 26 | $-0.827 \pm 0.450$ | 9 | $-0.002 \pm 0.623$ |
| 23 | $0.998 \pm 0.009$ | | |
| 18 | $-0.520 \pm 0.617$ | | |
| 9 | $-0.459 \pm 0.806$ | | |
| 8 | $-0.811 \pm 0.275$ | | |

[1] Wikipedia, "Impeachment of Dilma Rousseff," (2018), [Online; accessed 01-October-2018].
[2] Twitter Inc., "Filter realtime Tweets - Standard stream parameters," (2018), [Online; accessed 01-August-2018].
[3] M. Conover, B. Gonçalves, J. Ratkiewicz, A. Flammini, and F. Menczer, "Predicting the political alignment of Twitter users," in *Proceedings of 3rd IEEE Conference on Social Computing (SocialCom)* (2011).
[4] D. M. Romero, B. Meeder, and J. Kleinberg, "Differences in the mechanics of information diffusion across topics: Idioms, political hashtags, and complex contagion on Twitter," in *Proceedings of the 20th International Conference on World Wide Web*, WWW '11 (ACM, New York, NY, USA, 2011) pp. 695–704.
[5] A. Bessi, F. Zollo, M. Del Vicario, M. Puliga, A. Scala, G. Caldarelli, B. Uzzi, and W. Quattrociocchi, "Users polarization on Facebook and Youtube," PLOS ONE **11**, 1 (2016).
[6] M. D. Conover, B. Gonçalves, A. Flammini, and F. Menczer, "Partisan asymmetries in online political activity," EPJ Data Science **1**, 6 (2012).
[7] J. Borge-Holthoefer, W. Magdy, K. Darwish, and I. Weber, "Content and network dynamics behind egyptian political polarization on Twitter," in *Proceedings of the 18th ACM Conference on Computer Supported Cooperative Work & Social Computing*, CSCW '15 (ACM, New York, NY, USA, 2015) pp. 700–711.
[8] P. Holme and J. Saramäki, "Temporal networks," Physics Reports **519**, 97 (2012), temporal Networks.
[9] V. Nicosia, J. Tang, C. Mascolo, M. Musolesi, G. Russo, and V. Latora, "Graph metrics for temporal networks," in *Temporal networks* (Springer, 2013) pp. 15–40.
[10] R. Tarjan, "Depth-first search and linear graph algorithms," SIAM Journal on Computing **1**, 146 (1972).
[11] E. Nuutila and E. Soisalon-Soininen, "On finding the strongly connected components in a directed graph," Information Processing Letters **49**, 9 (1994).
[12] S. Fortunato, "Community detection in graphs," Physics Reports **486**, 75 (2010).
[13] V. D. Blondel, J.-L. Guillaume, R. Lambiotte, and E. Lefebvre, "Fast unfolding of communities in large networks," Journal of Statistical Mechanics: Theory and Experiment **2008**, P10008 (2008).
[14] S. N. Dorogovtsev, A. V. Goltsev, and J. F. F. Mendes, "$k$-core organization of complex networks," Phys. Rev. Lett. **96**, 040601 (2006).
[15] D. J. Watts, "A simple model of global cascades on random networks," Proceedings of the National Academy of Sciences **99**, 5766 (2002).
[16] F. Karimi and P. Holme, "Threshold model of cascades in empirical temporal networks," Physica A: Statistical Mechanics and its Applications **392**, 3476 (2013).
[17] S. Fortunato and M. Barthelemy, "Resolution limit in community detection," Proc. Natl. Acad. Sci. **104**, 36 (2007).
